# Supplementary material for: Towards a characterization of X-ray galaxy clusters for cosmology
Source: arXiv:1907.03806 ancillary file (2019-07-08)
Supplement: Supplementary file 1 [file appendix.pdf]

## Appendix D: HIFLUGCS images and surface brightness profiles

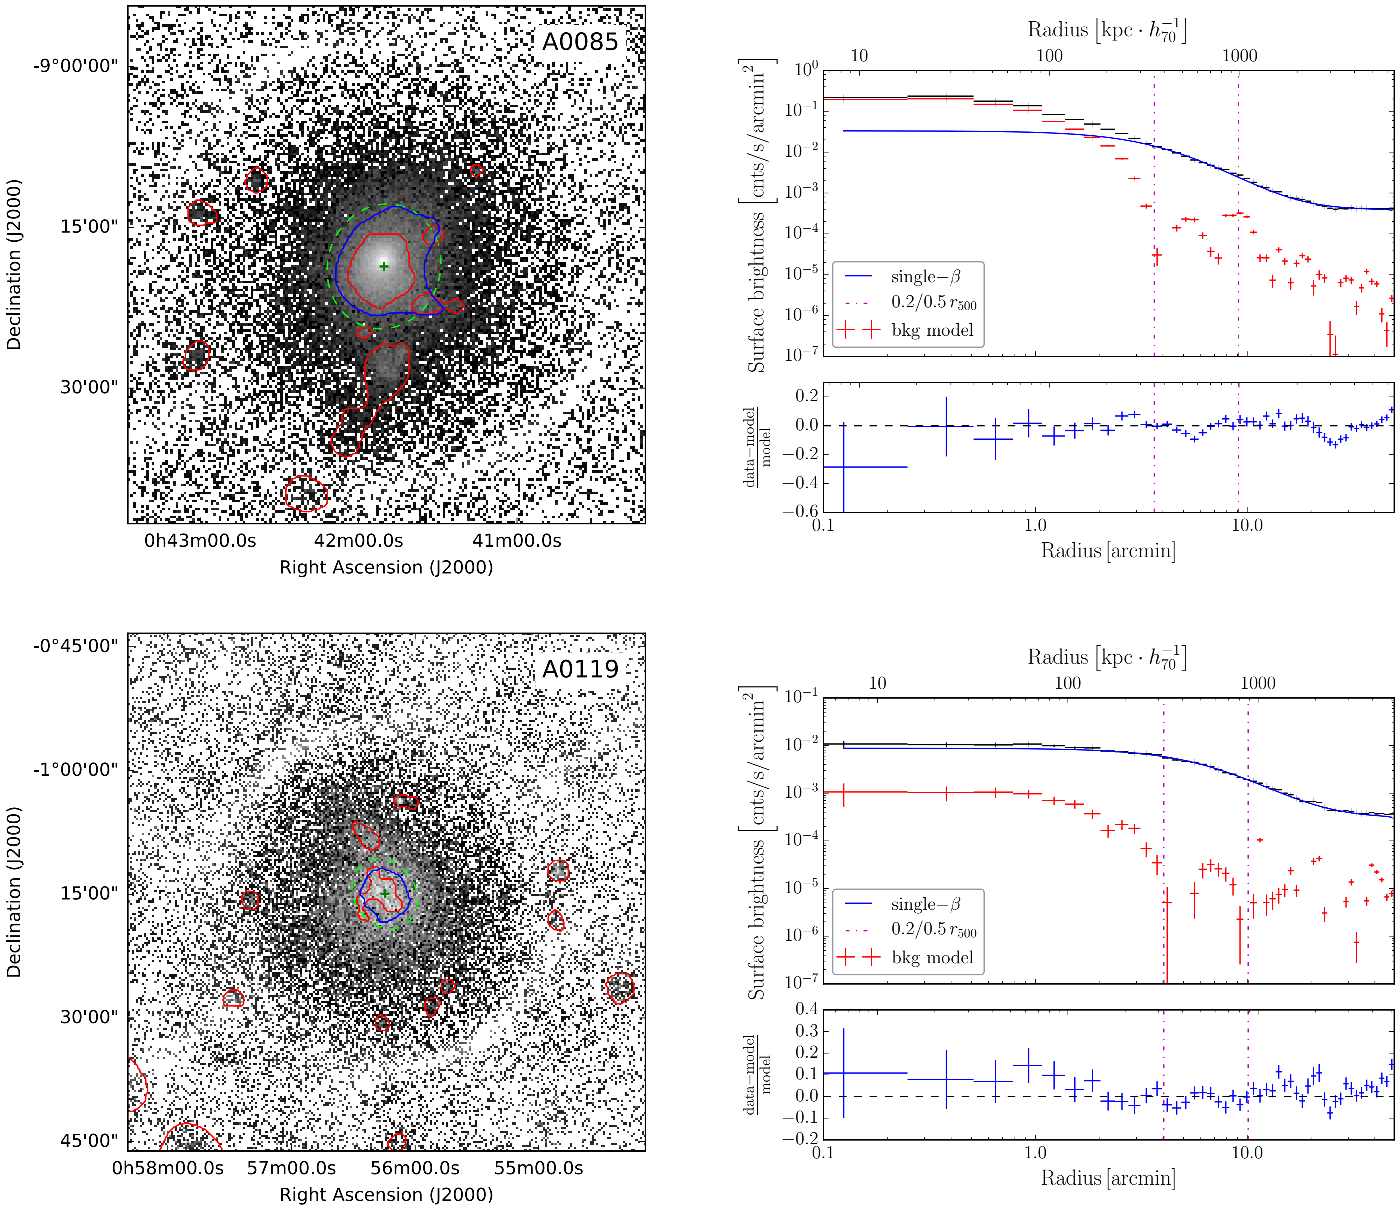


Fig. D.1: *Left*: ROSAT count rate images for individual galaxy clusters. The large scale centres are shown as *green plus signs*. *Red* contours correspond to wavelet scales used for background modelling. The large scales (the ones above 0.2 $r_{500}$) are shown as *blue* contours. These large scales are used to calculate the center and ellipticities. The extracted SExtractor ellipses are displayed in dashed green. Each box size corresponds to the outer significance radius of the shown cluster. *Right*: The *upper panels* show the measured (*black points*) surface brightness profiles of individual galaxy clusters. The background models used for the single $\beta$-model fits (*solid blue lines*) are shown as *red points*. The *lower panels* show the residuals of the core-modelled single $\beta$-model fits.

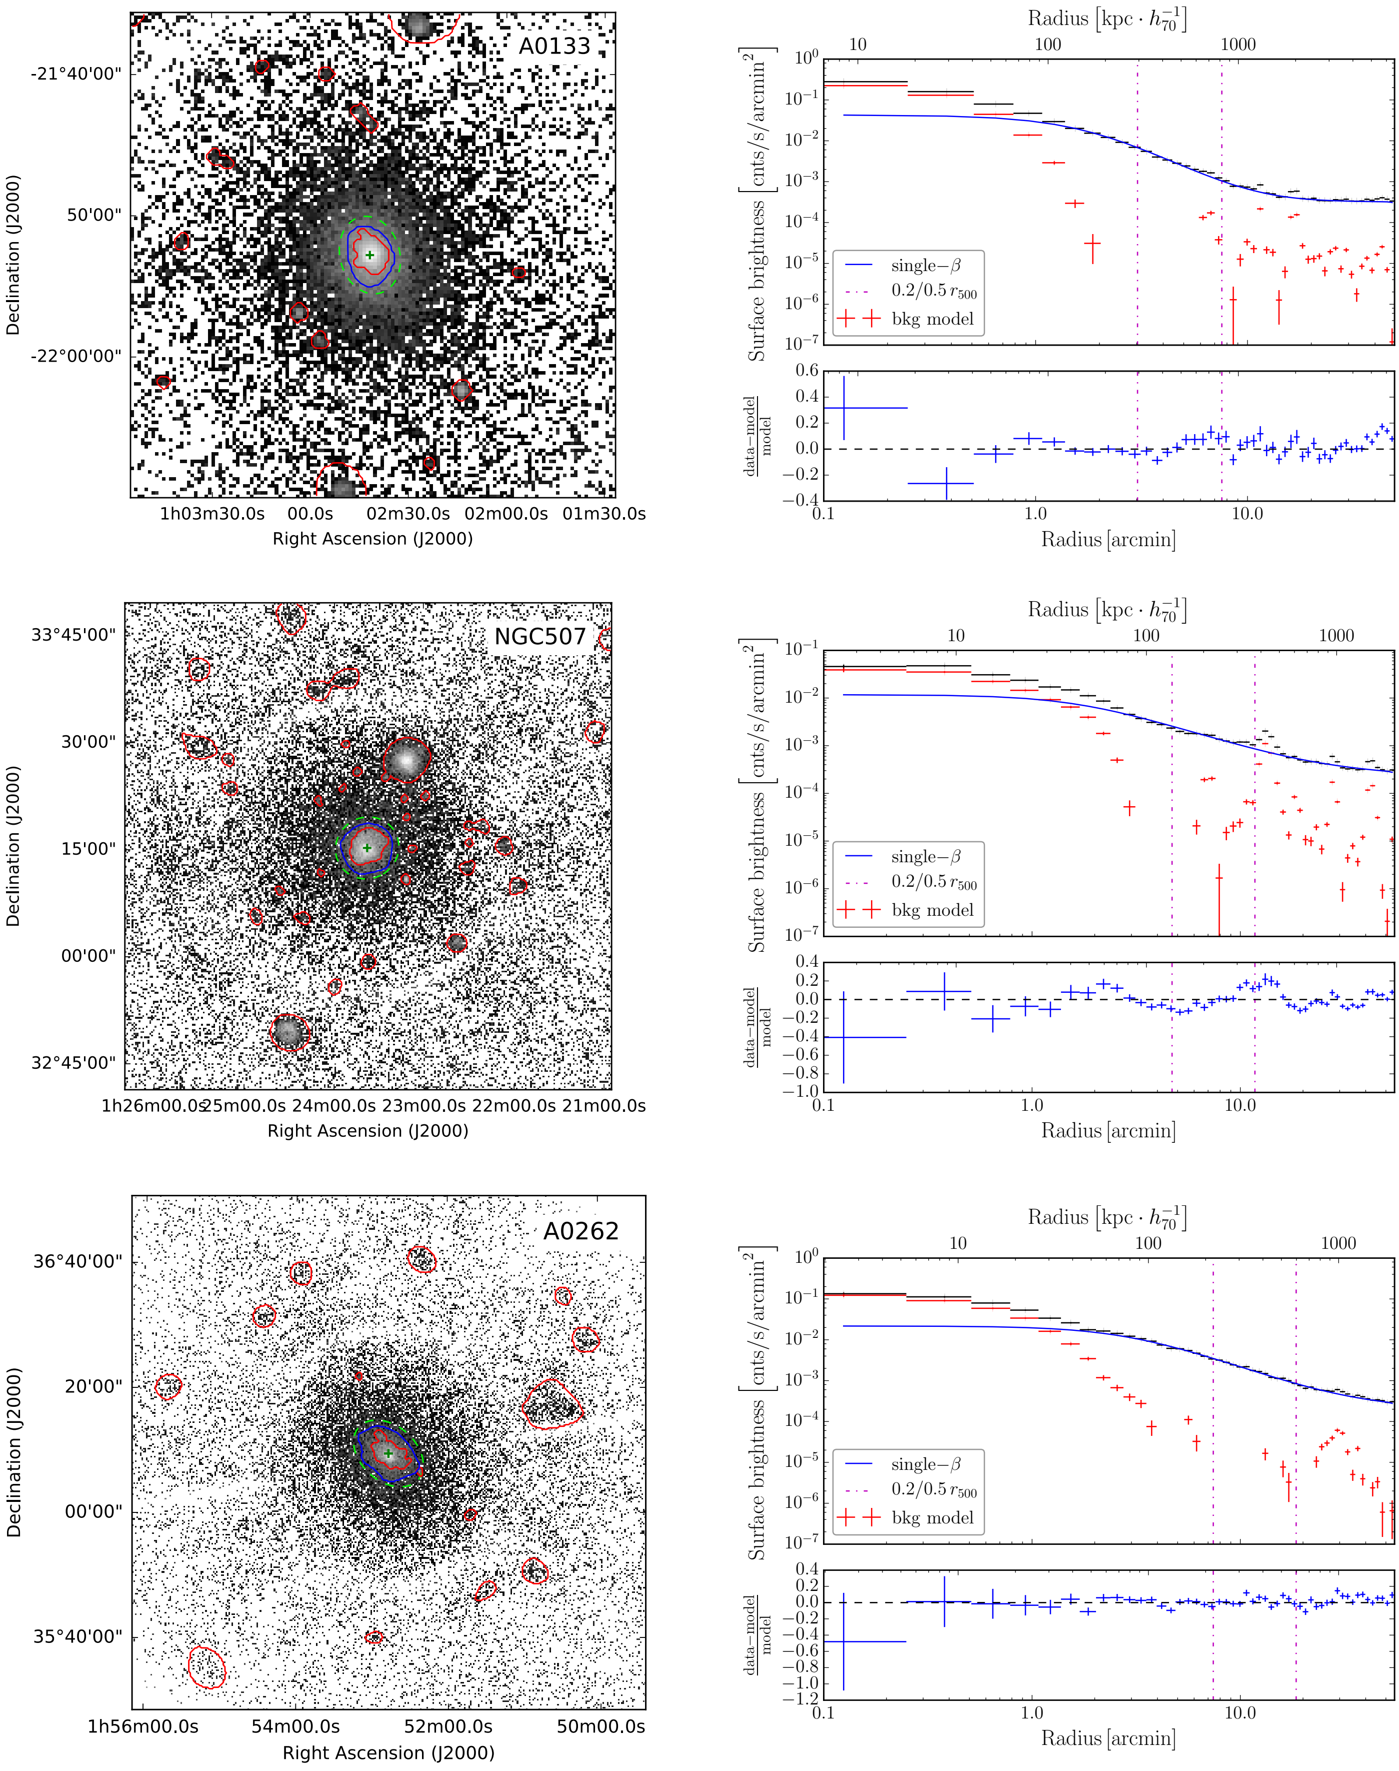


Fig. D.1: Continued.

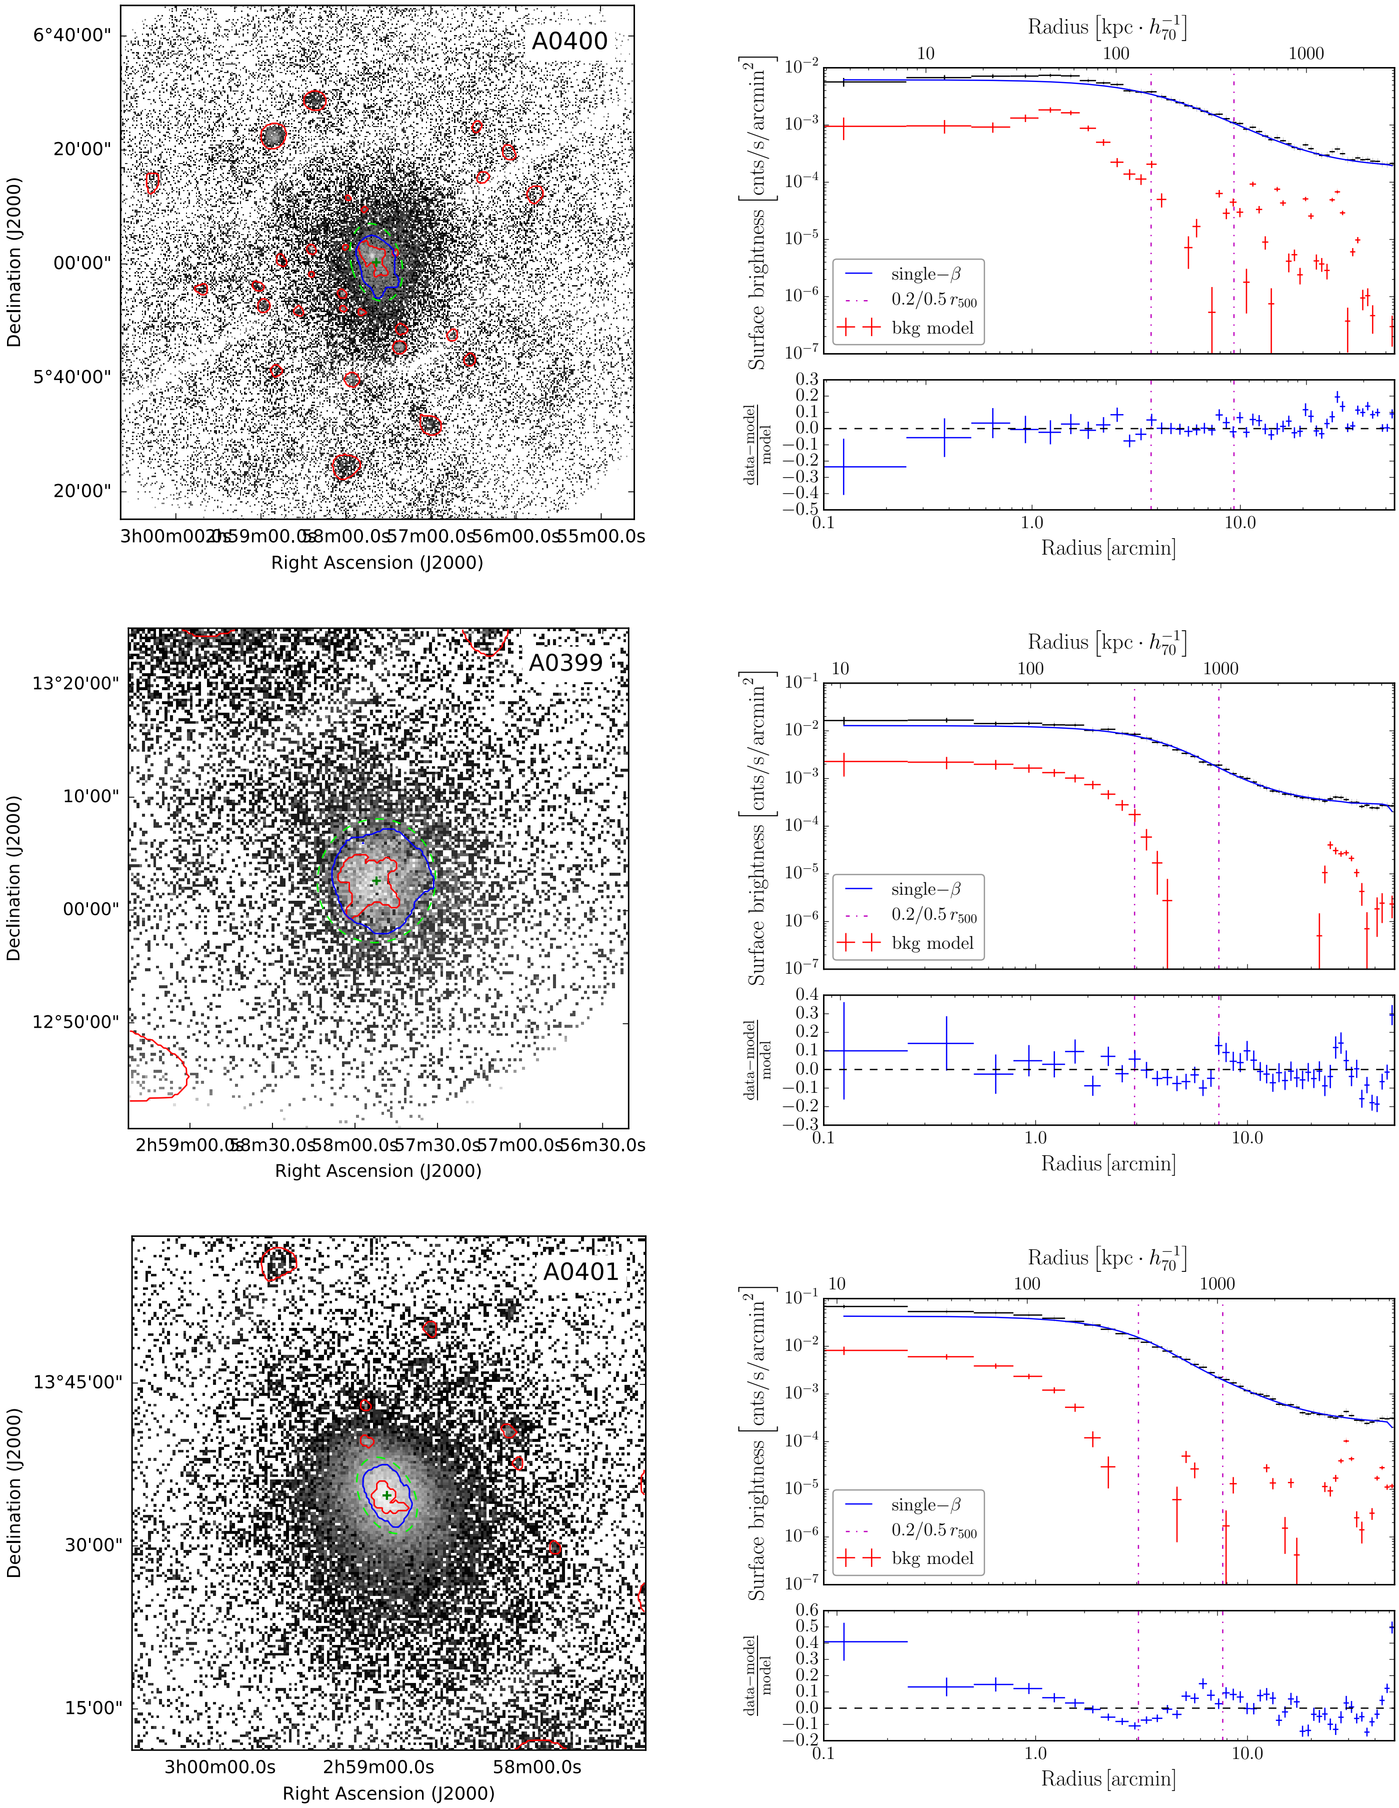


Fig. D.1: Continued.

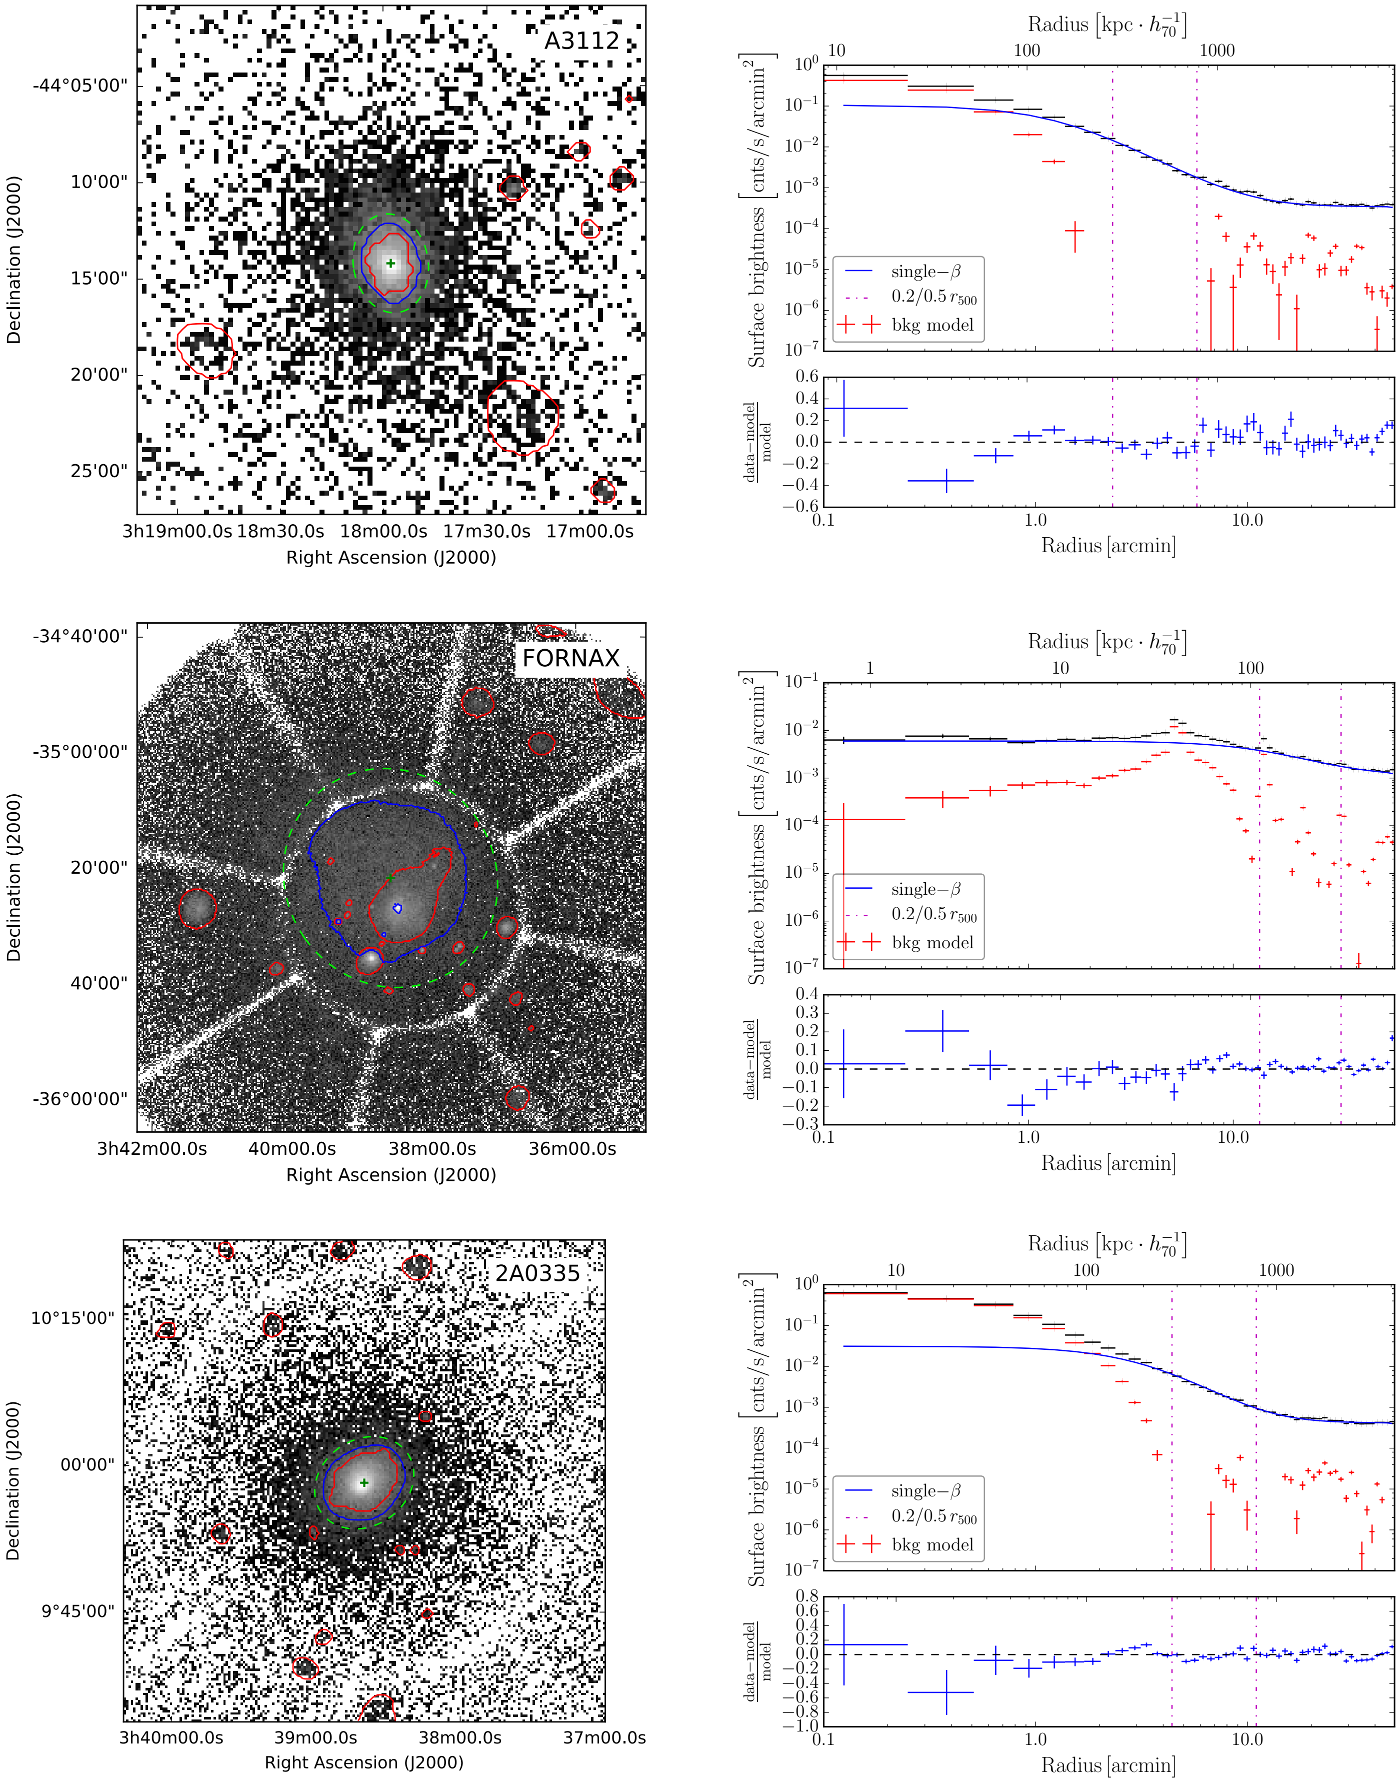


Fig. D.1: Continued.

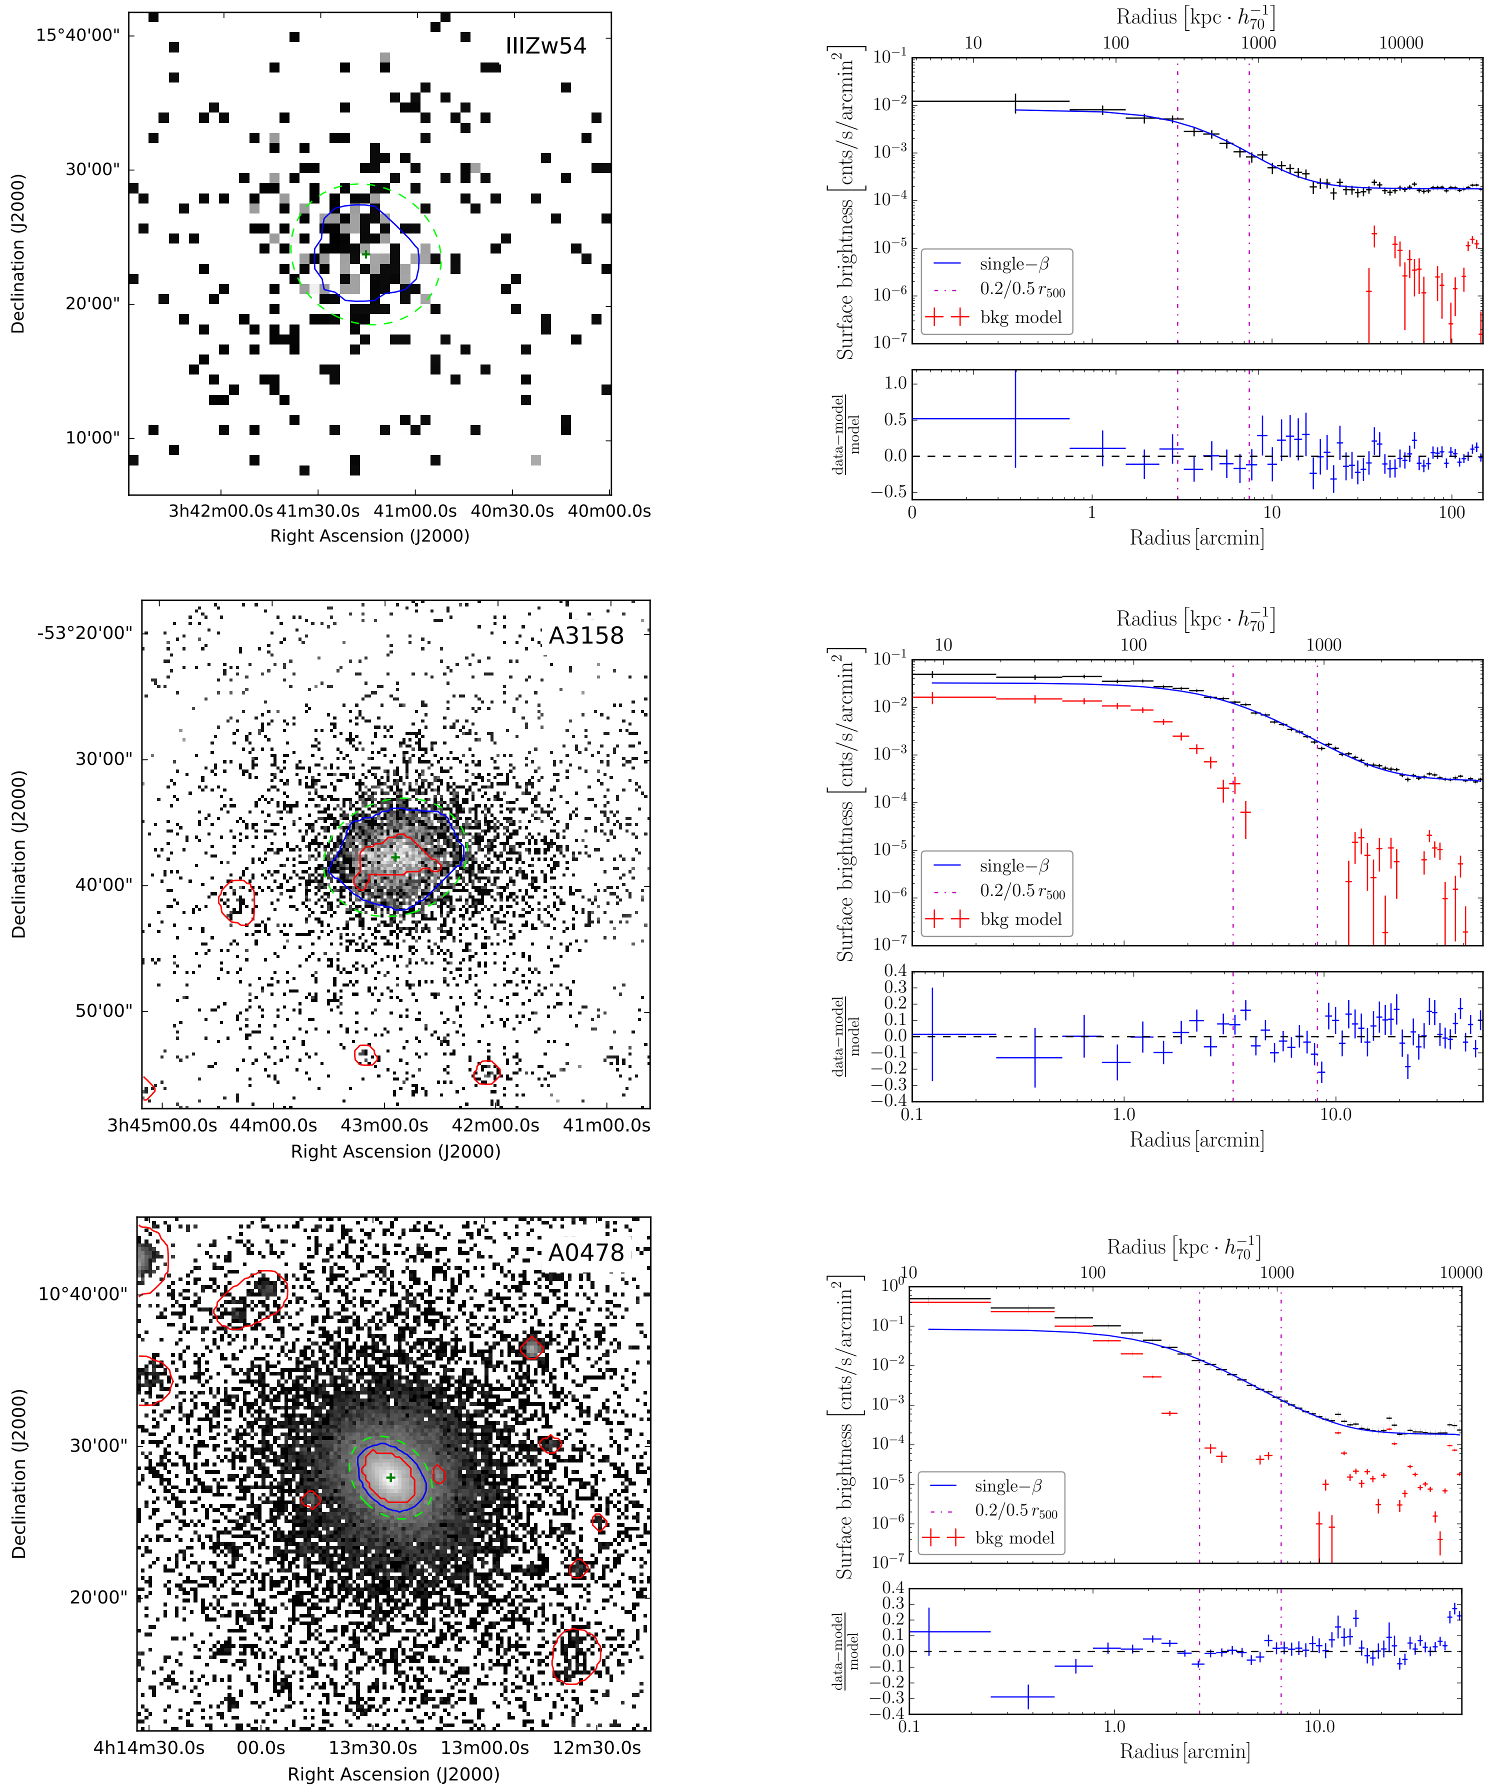


Fig. D.1: Continued.

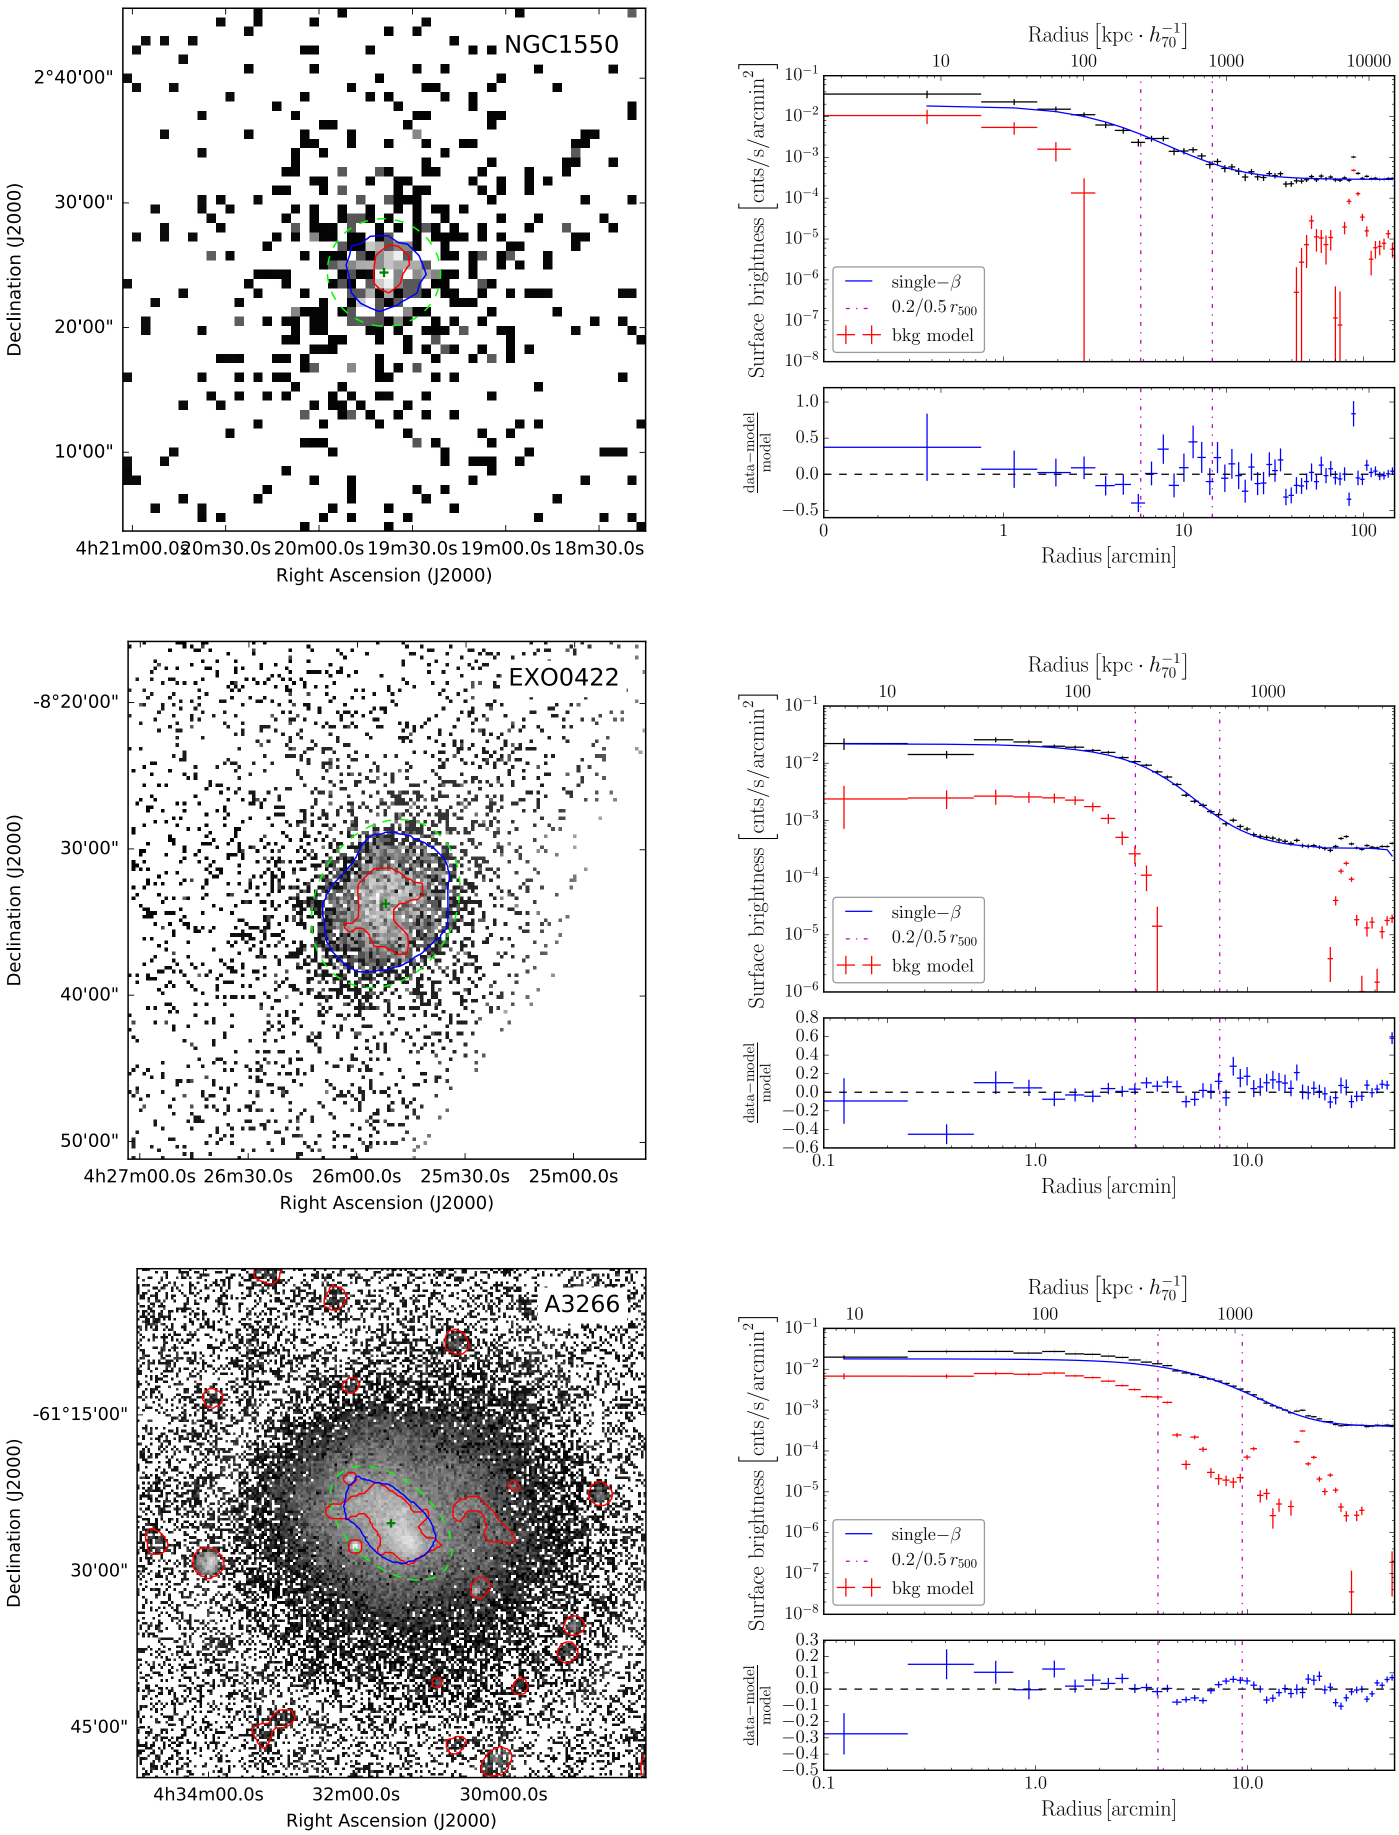


Fig. D.1: Continued.

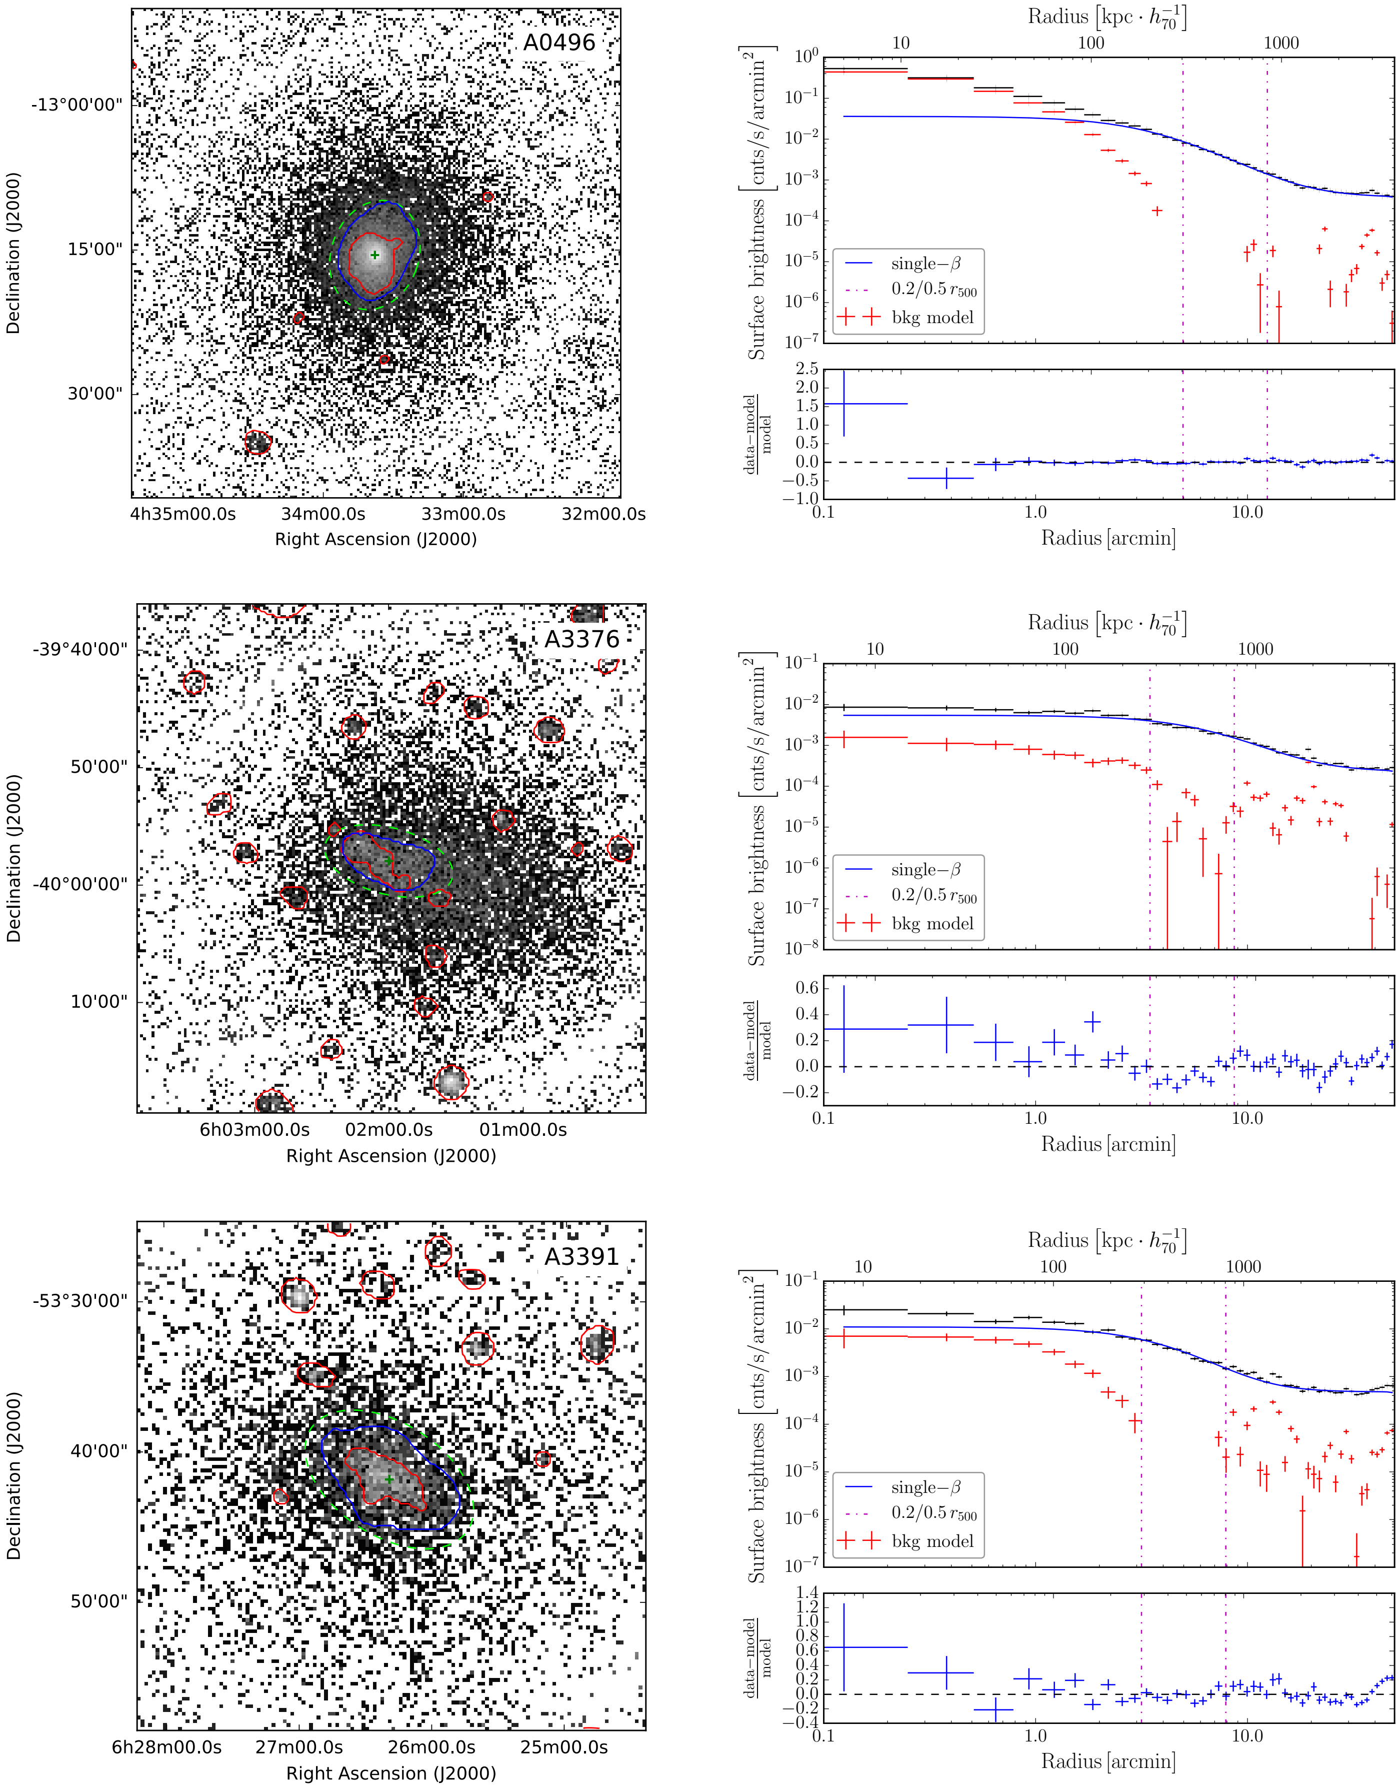


Fig. D.1: Continued.

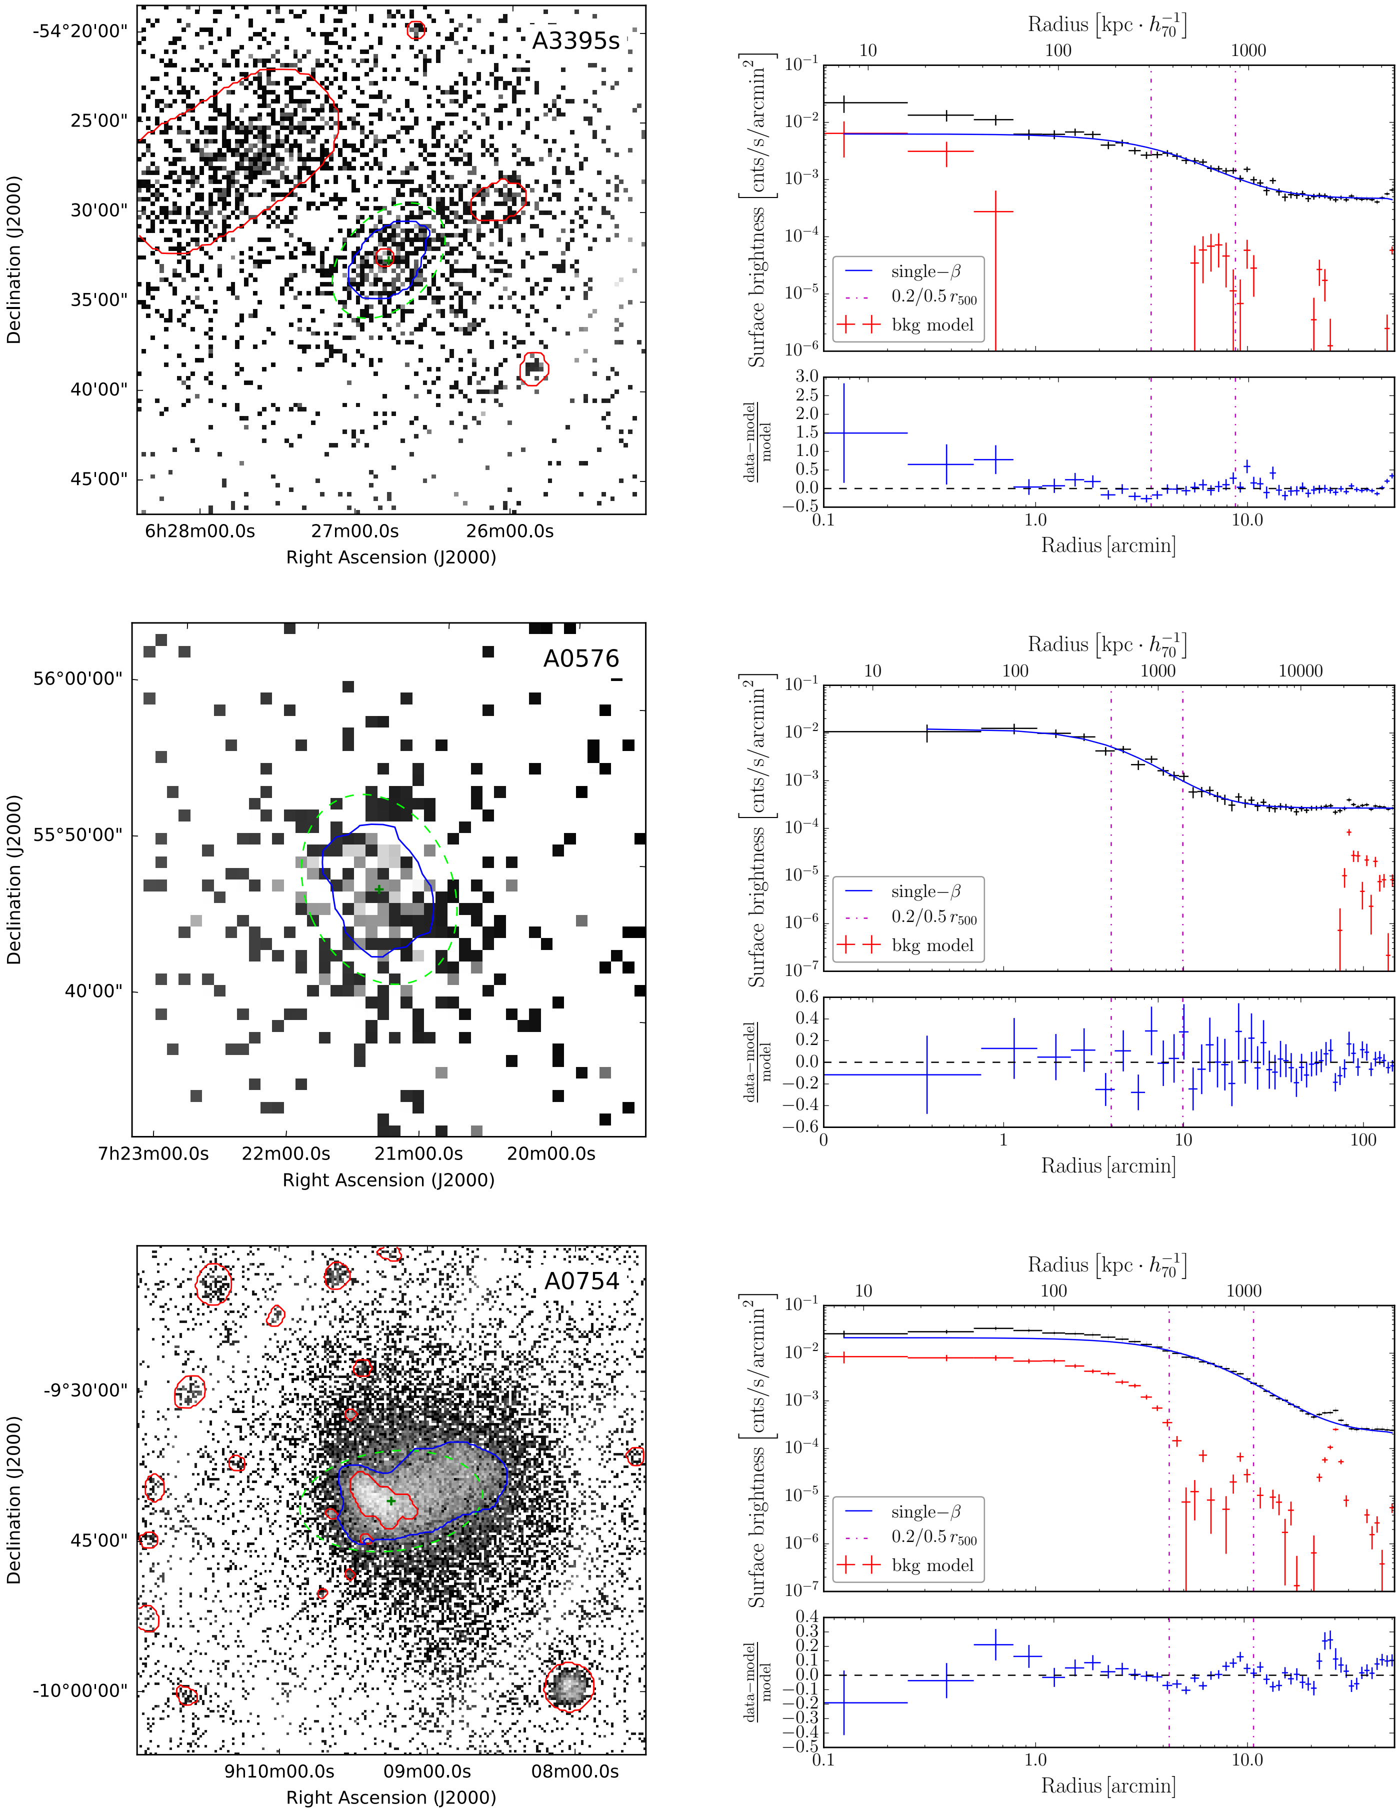


Fig. D.1: Continued.

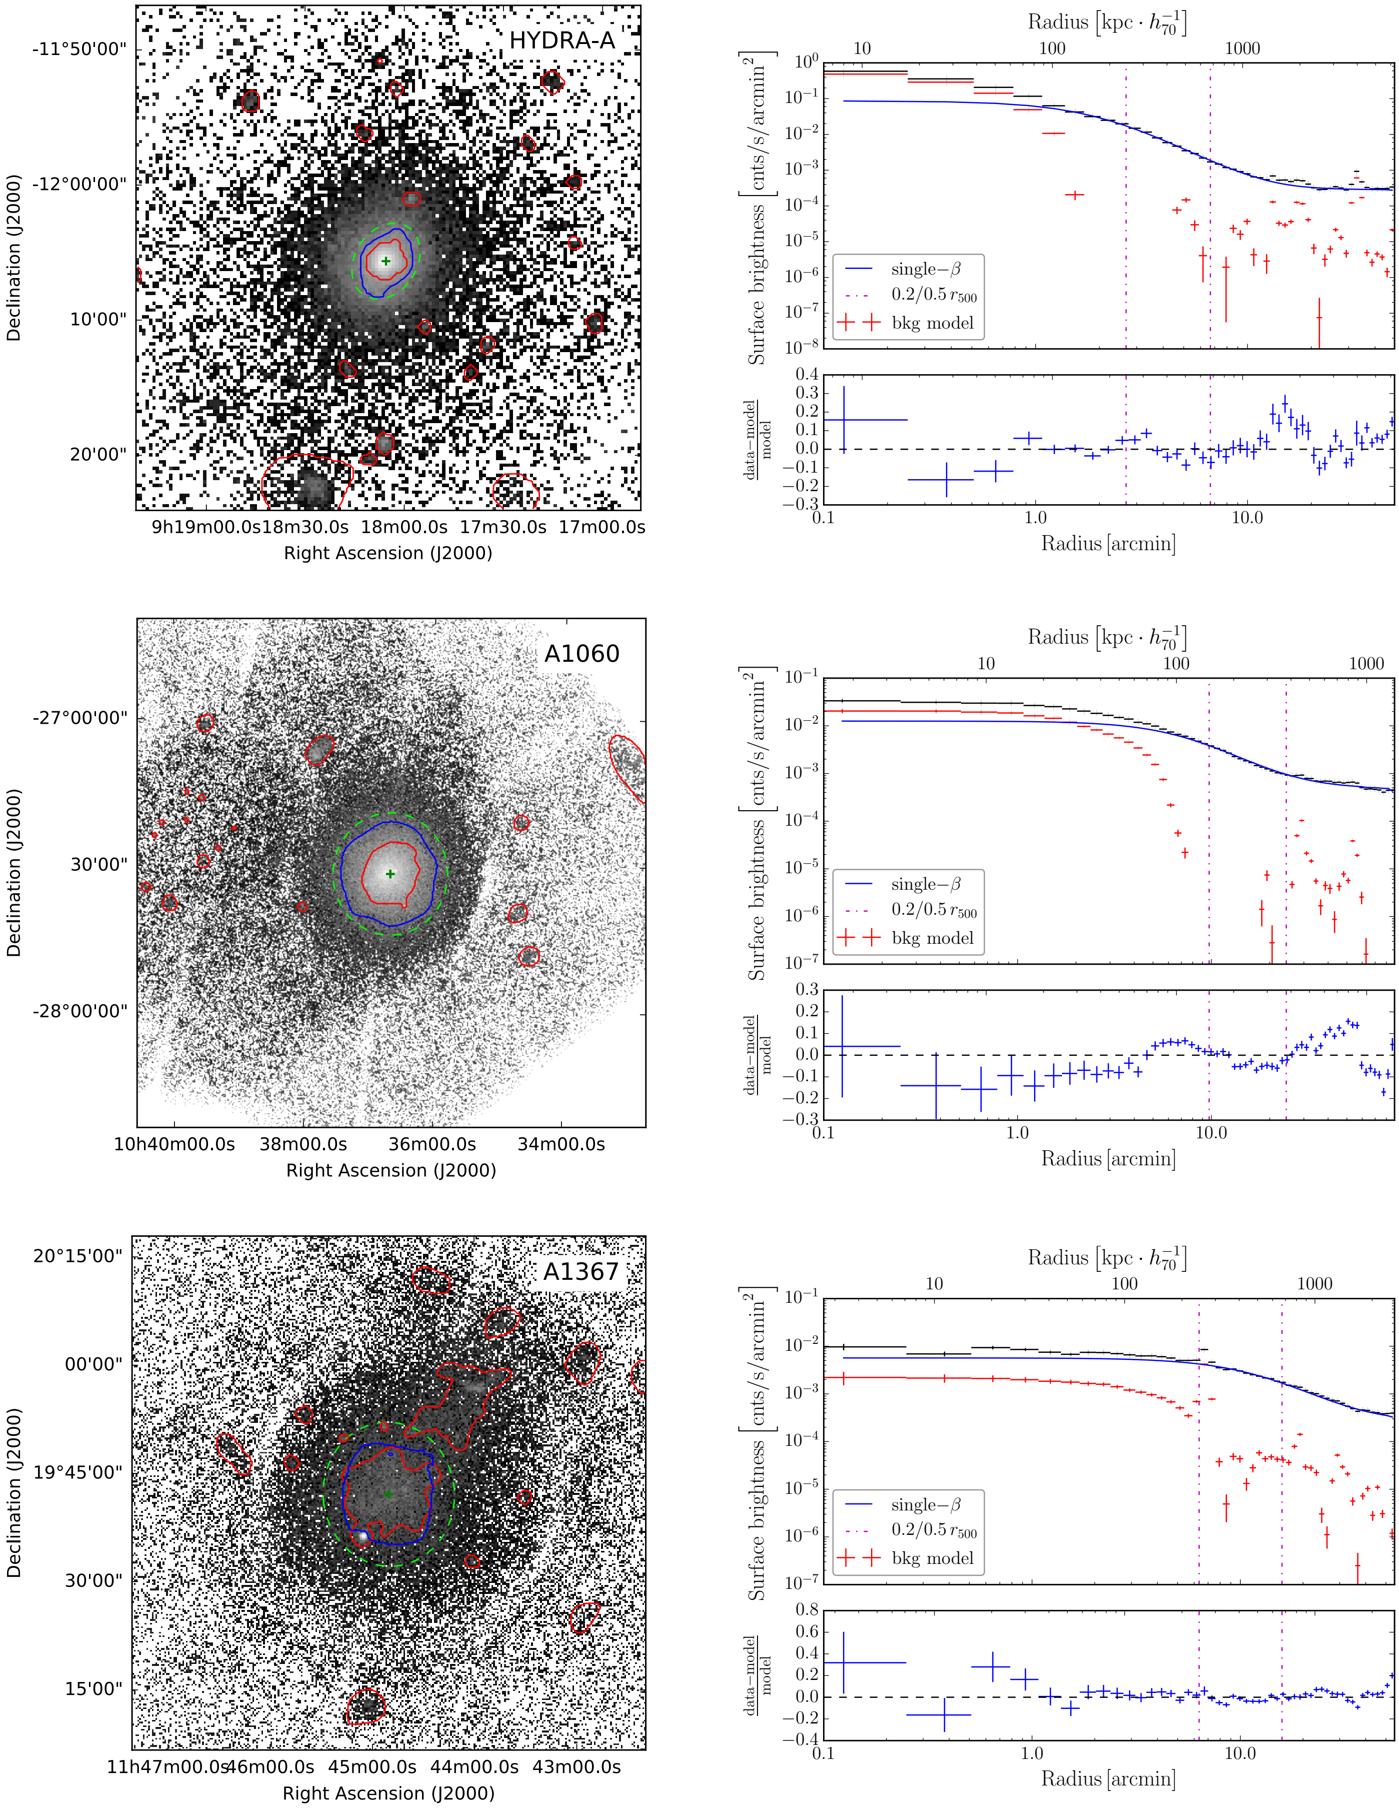


Fig. D.1: Continued.

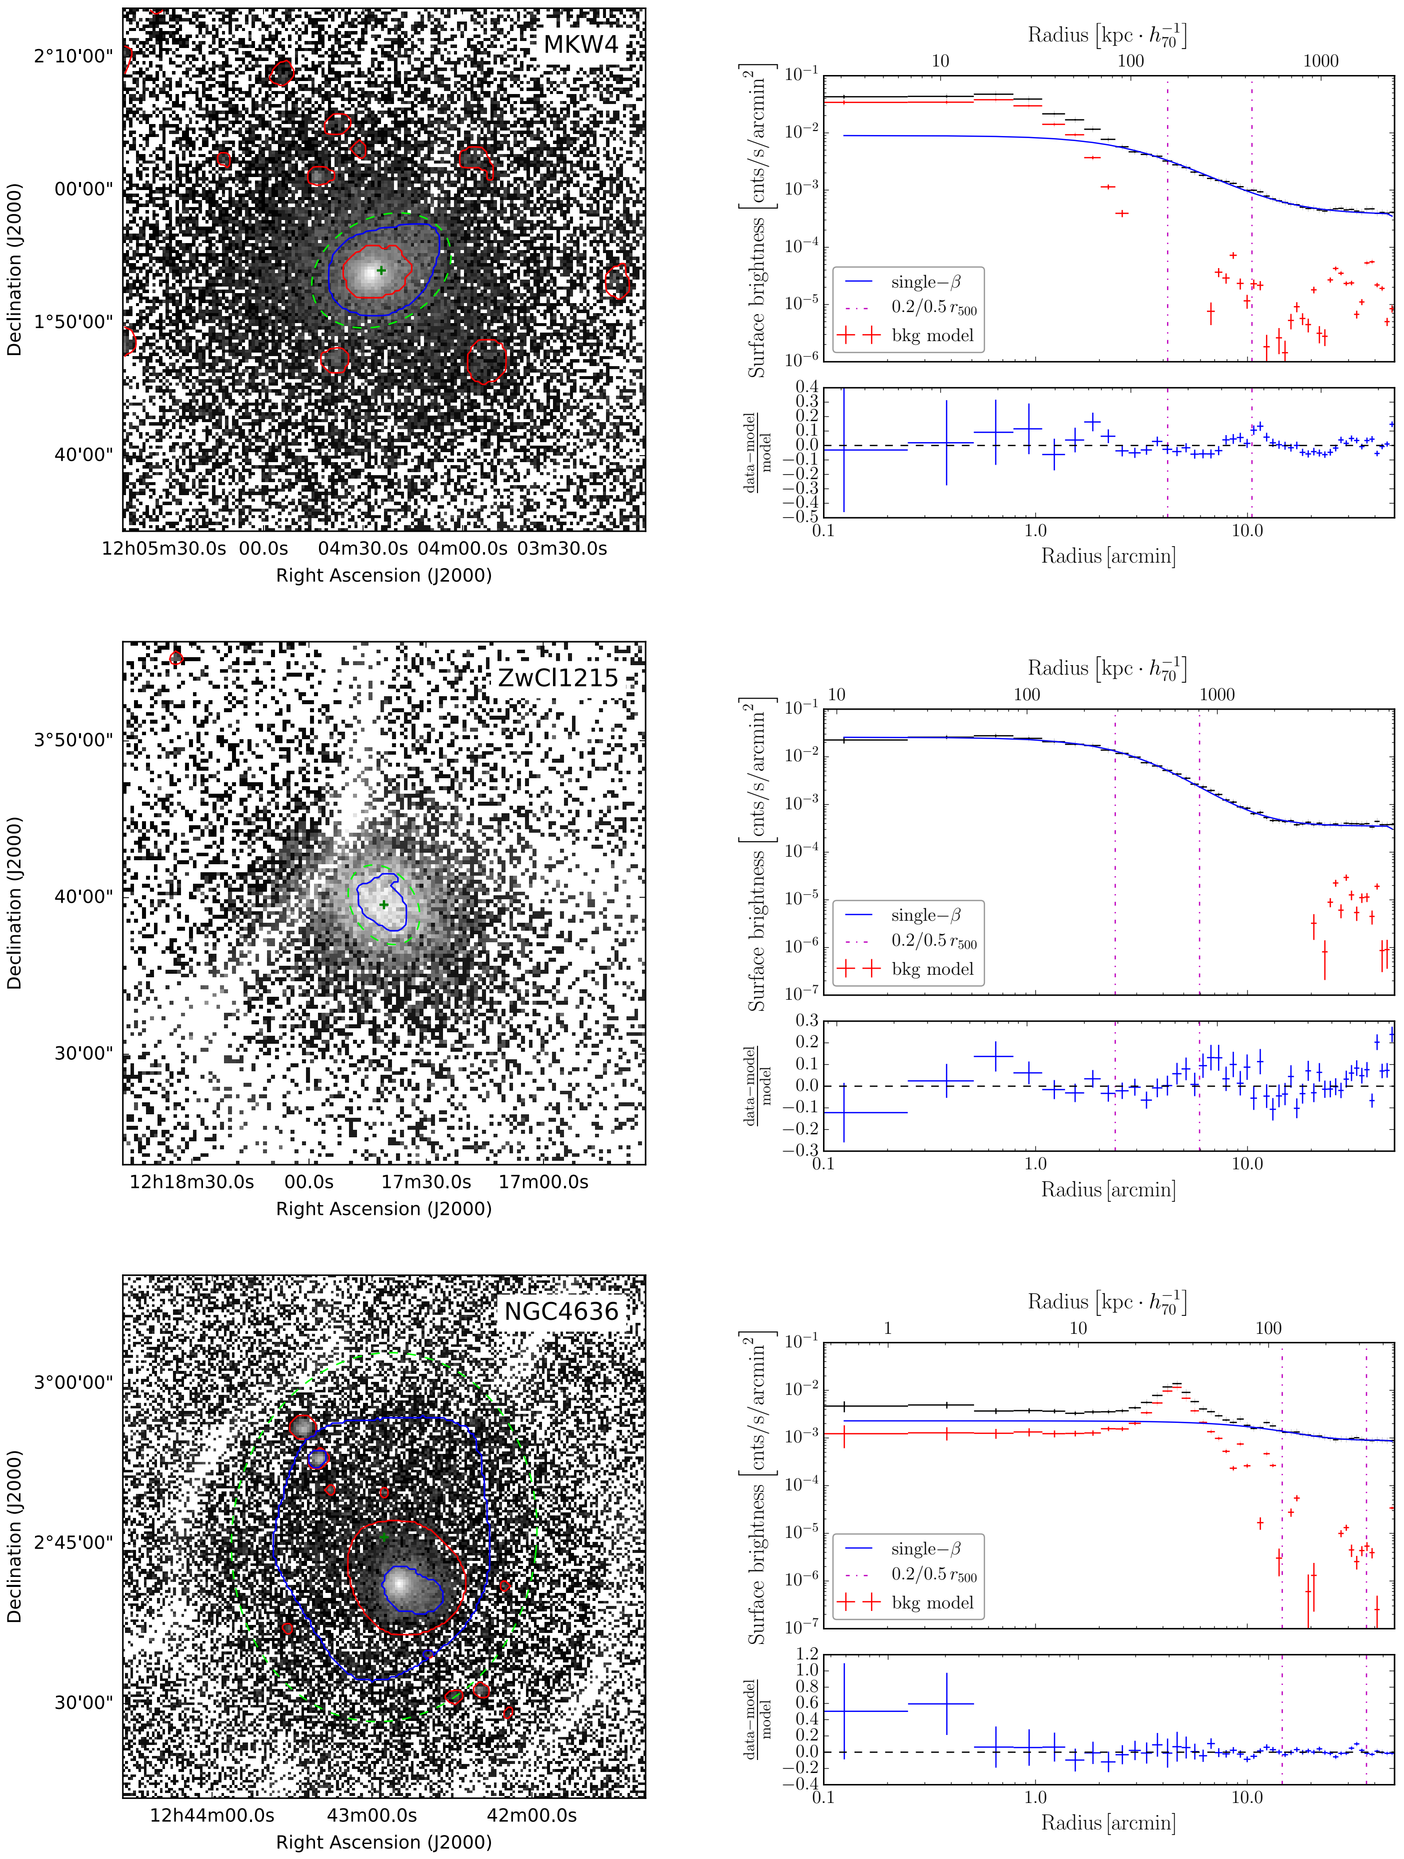


Fig. D.1: Continued.

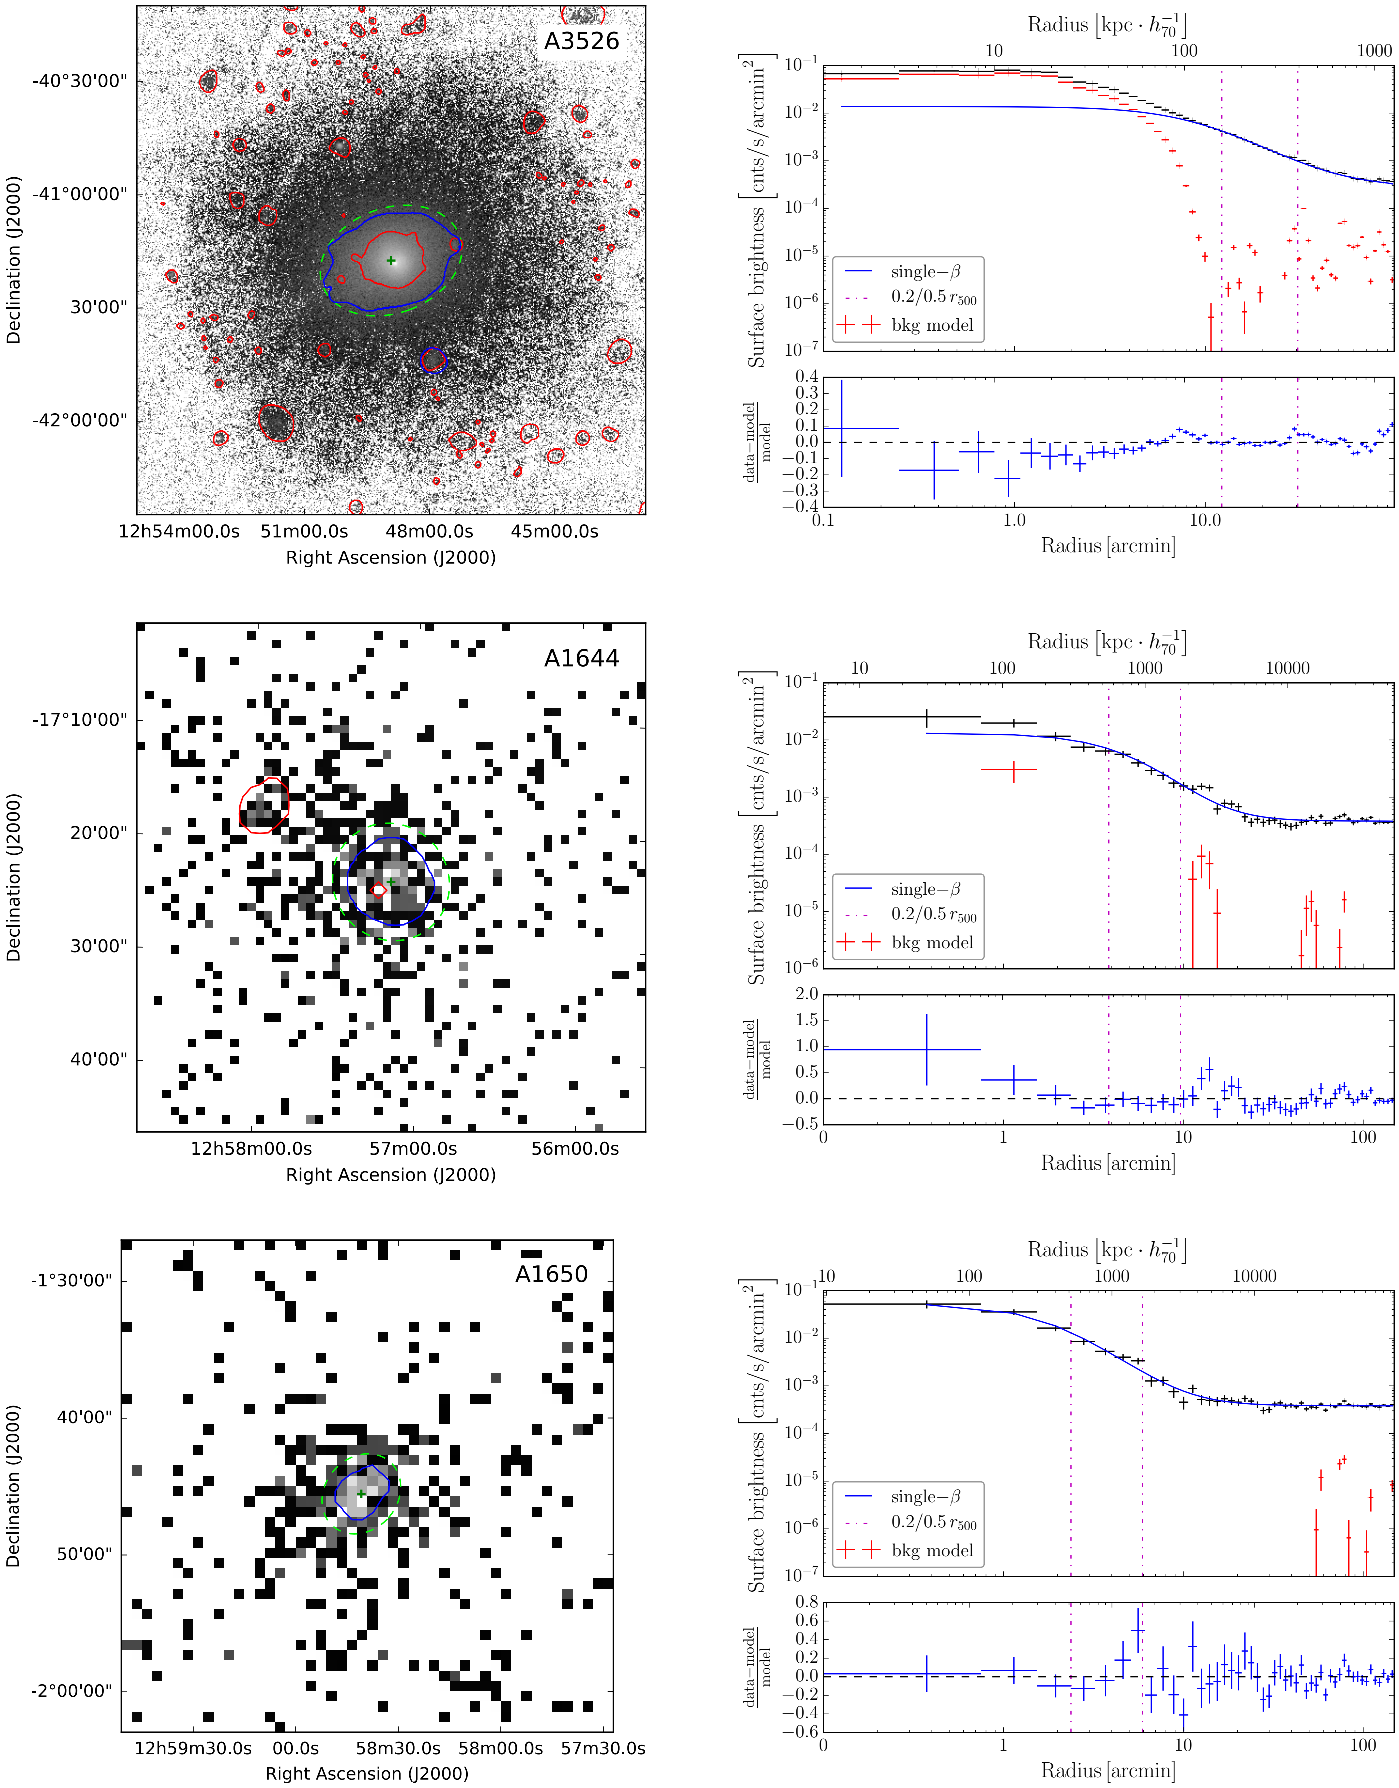


Fig. D.1: Continued.

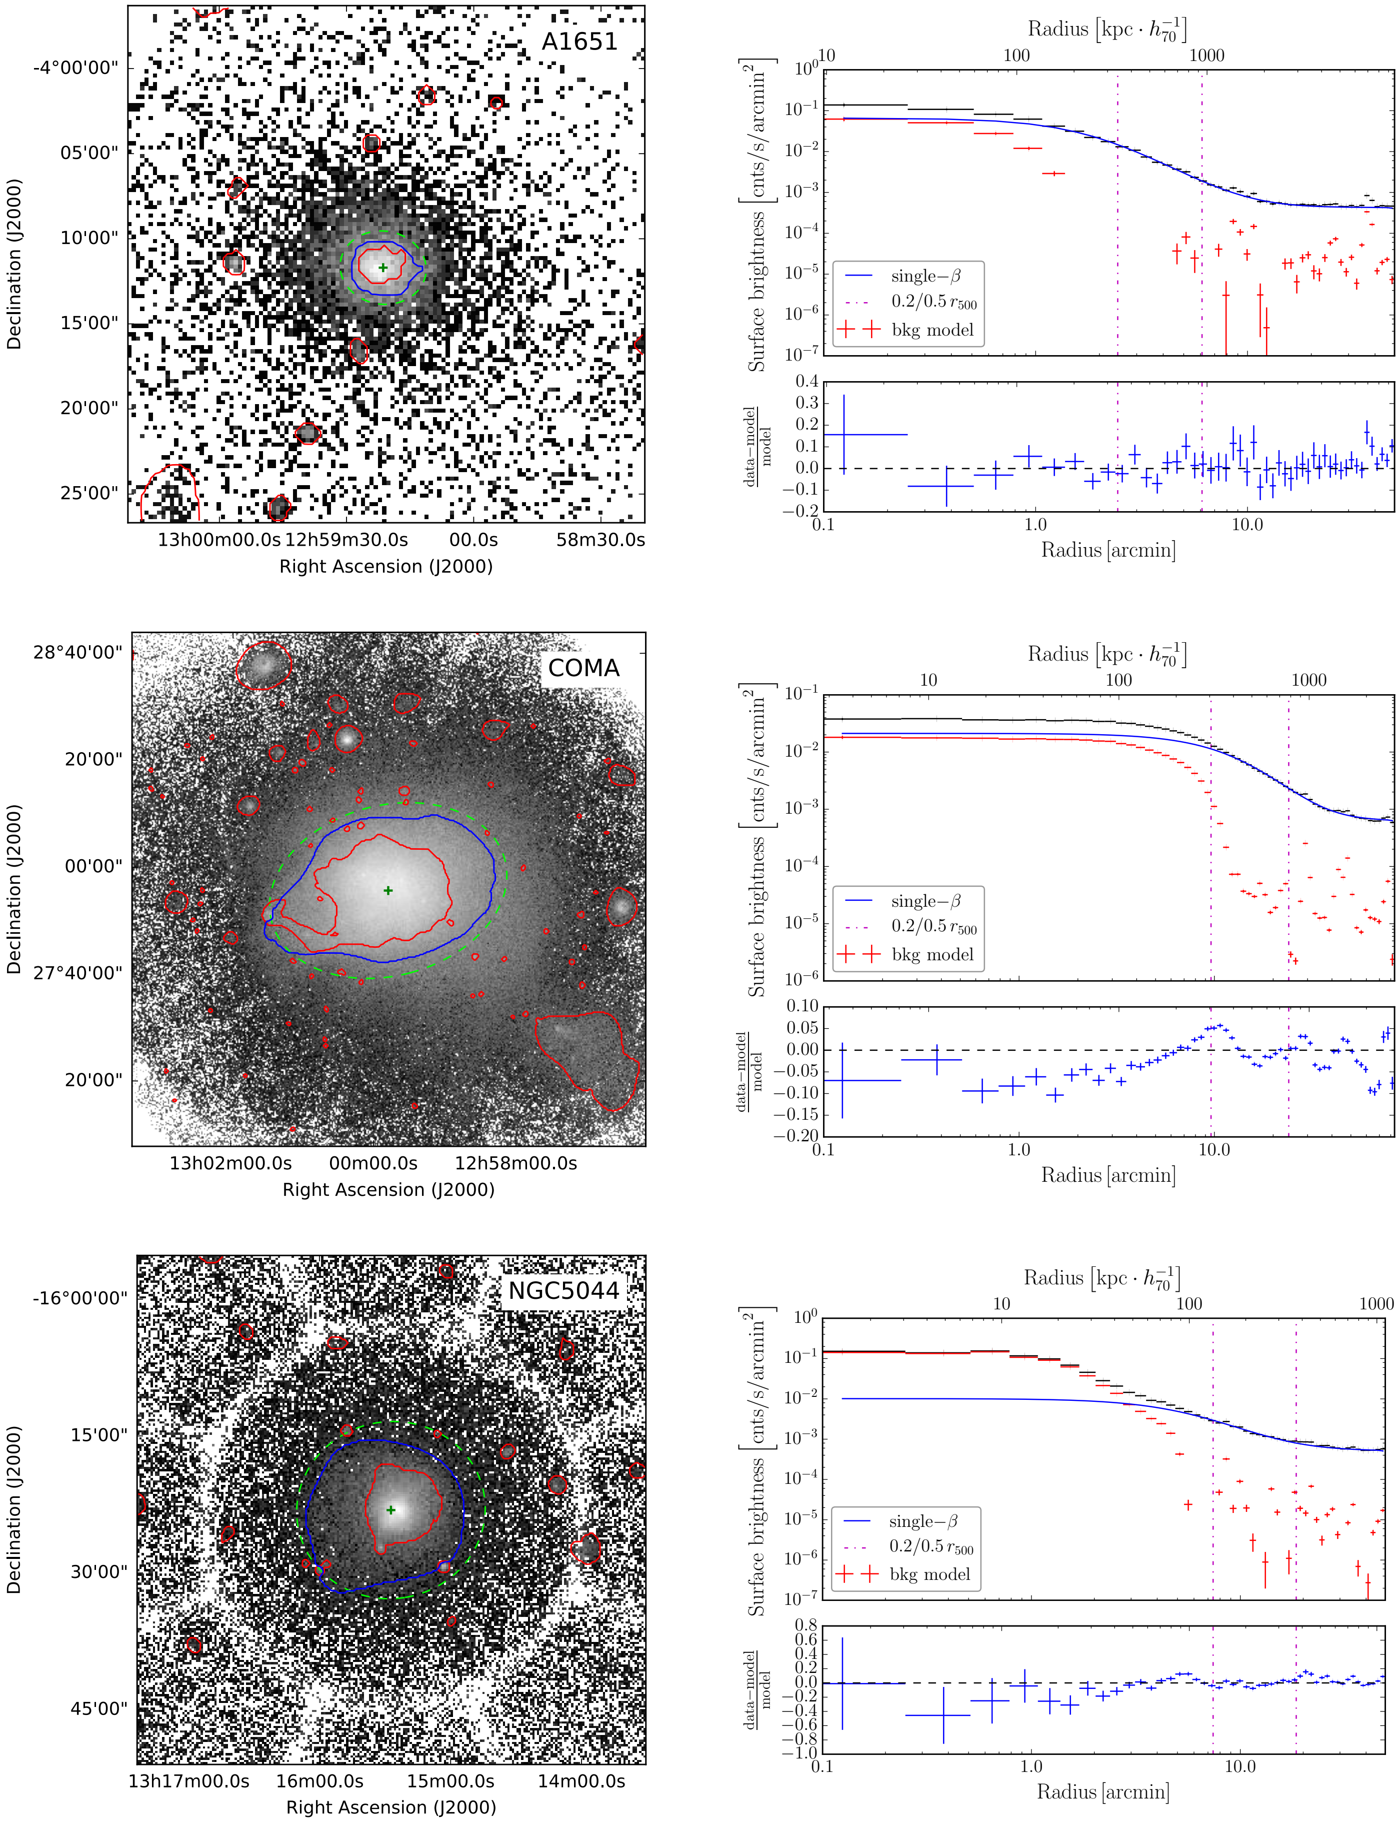


Fig. D.1: Continued.

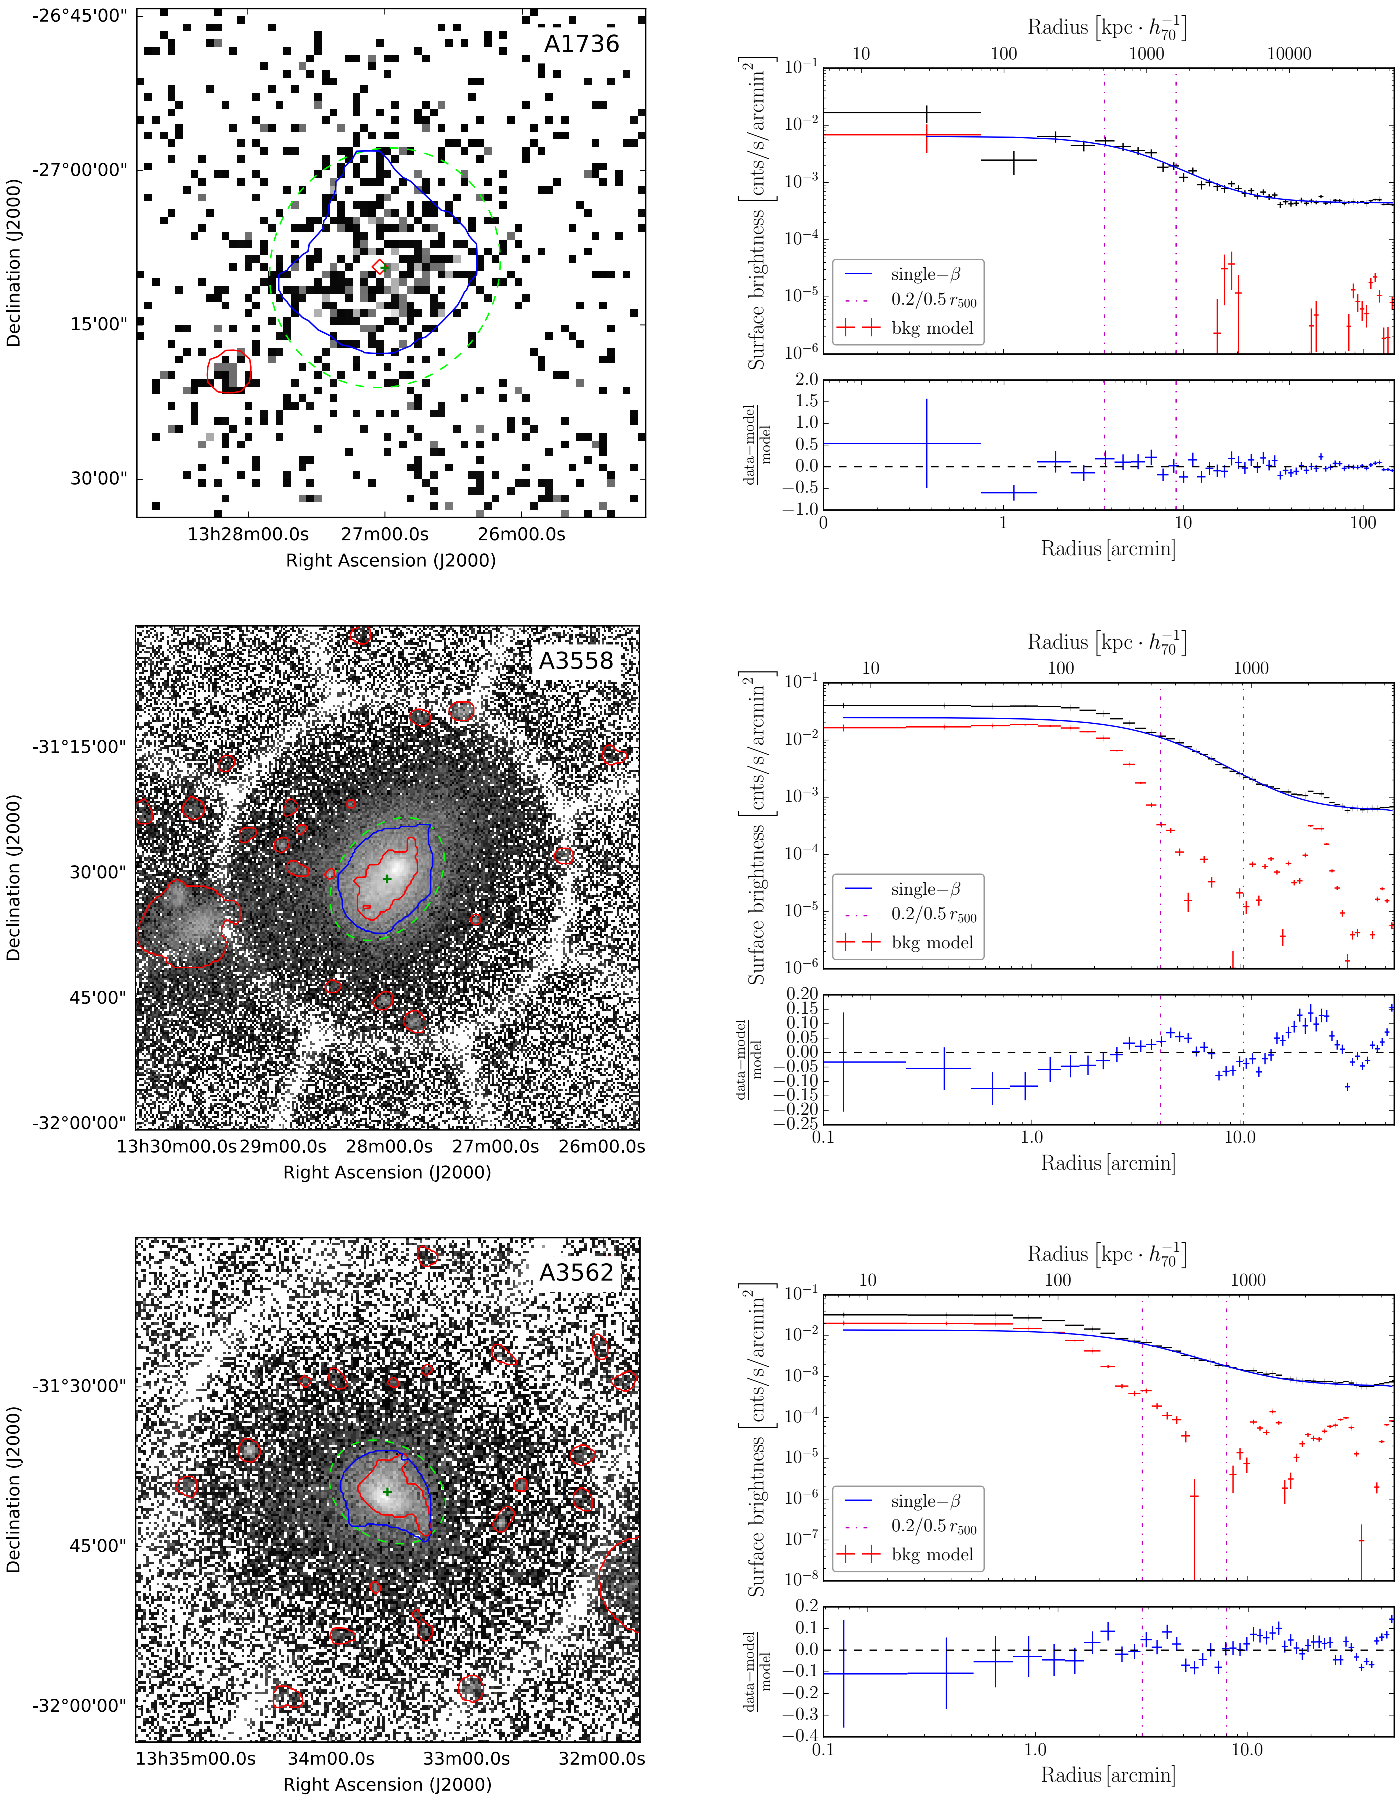


Fig. D.1: Continued.

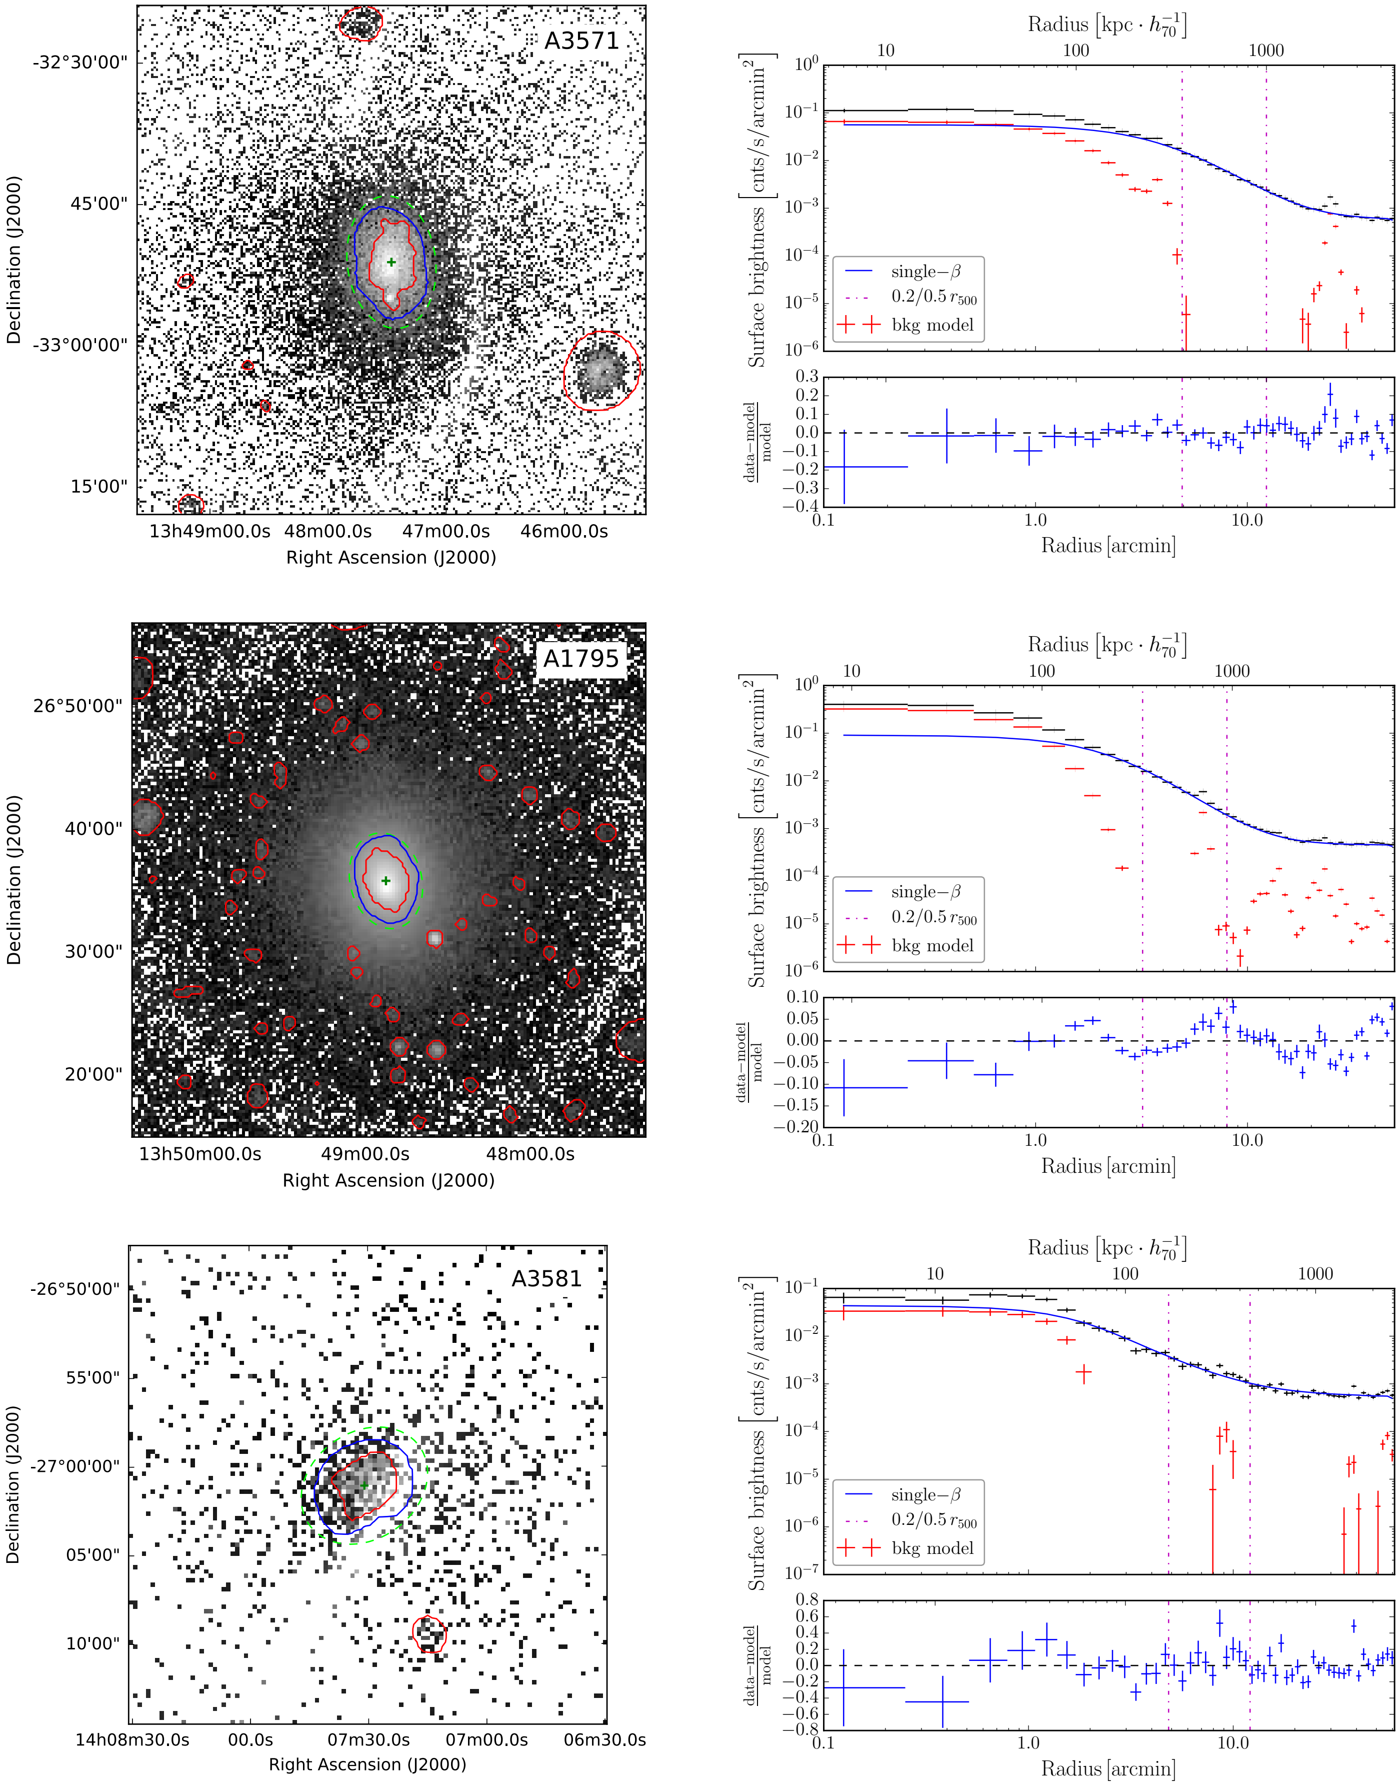


Fig. D.1: Continued.

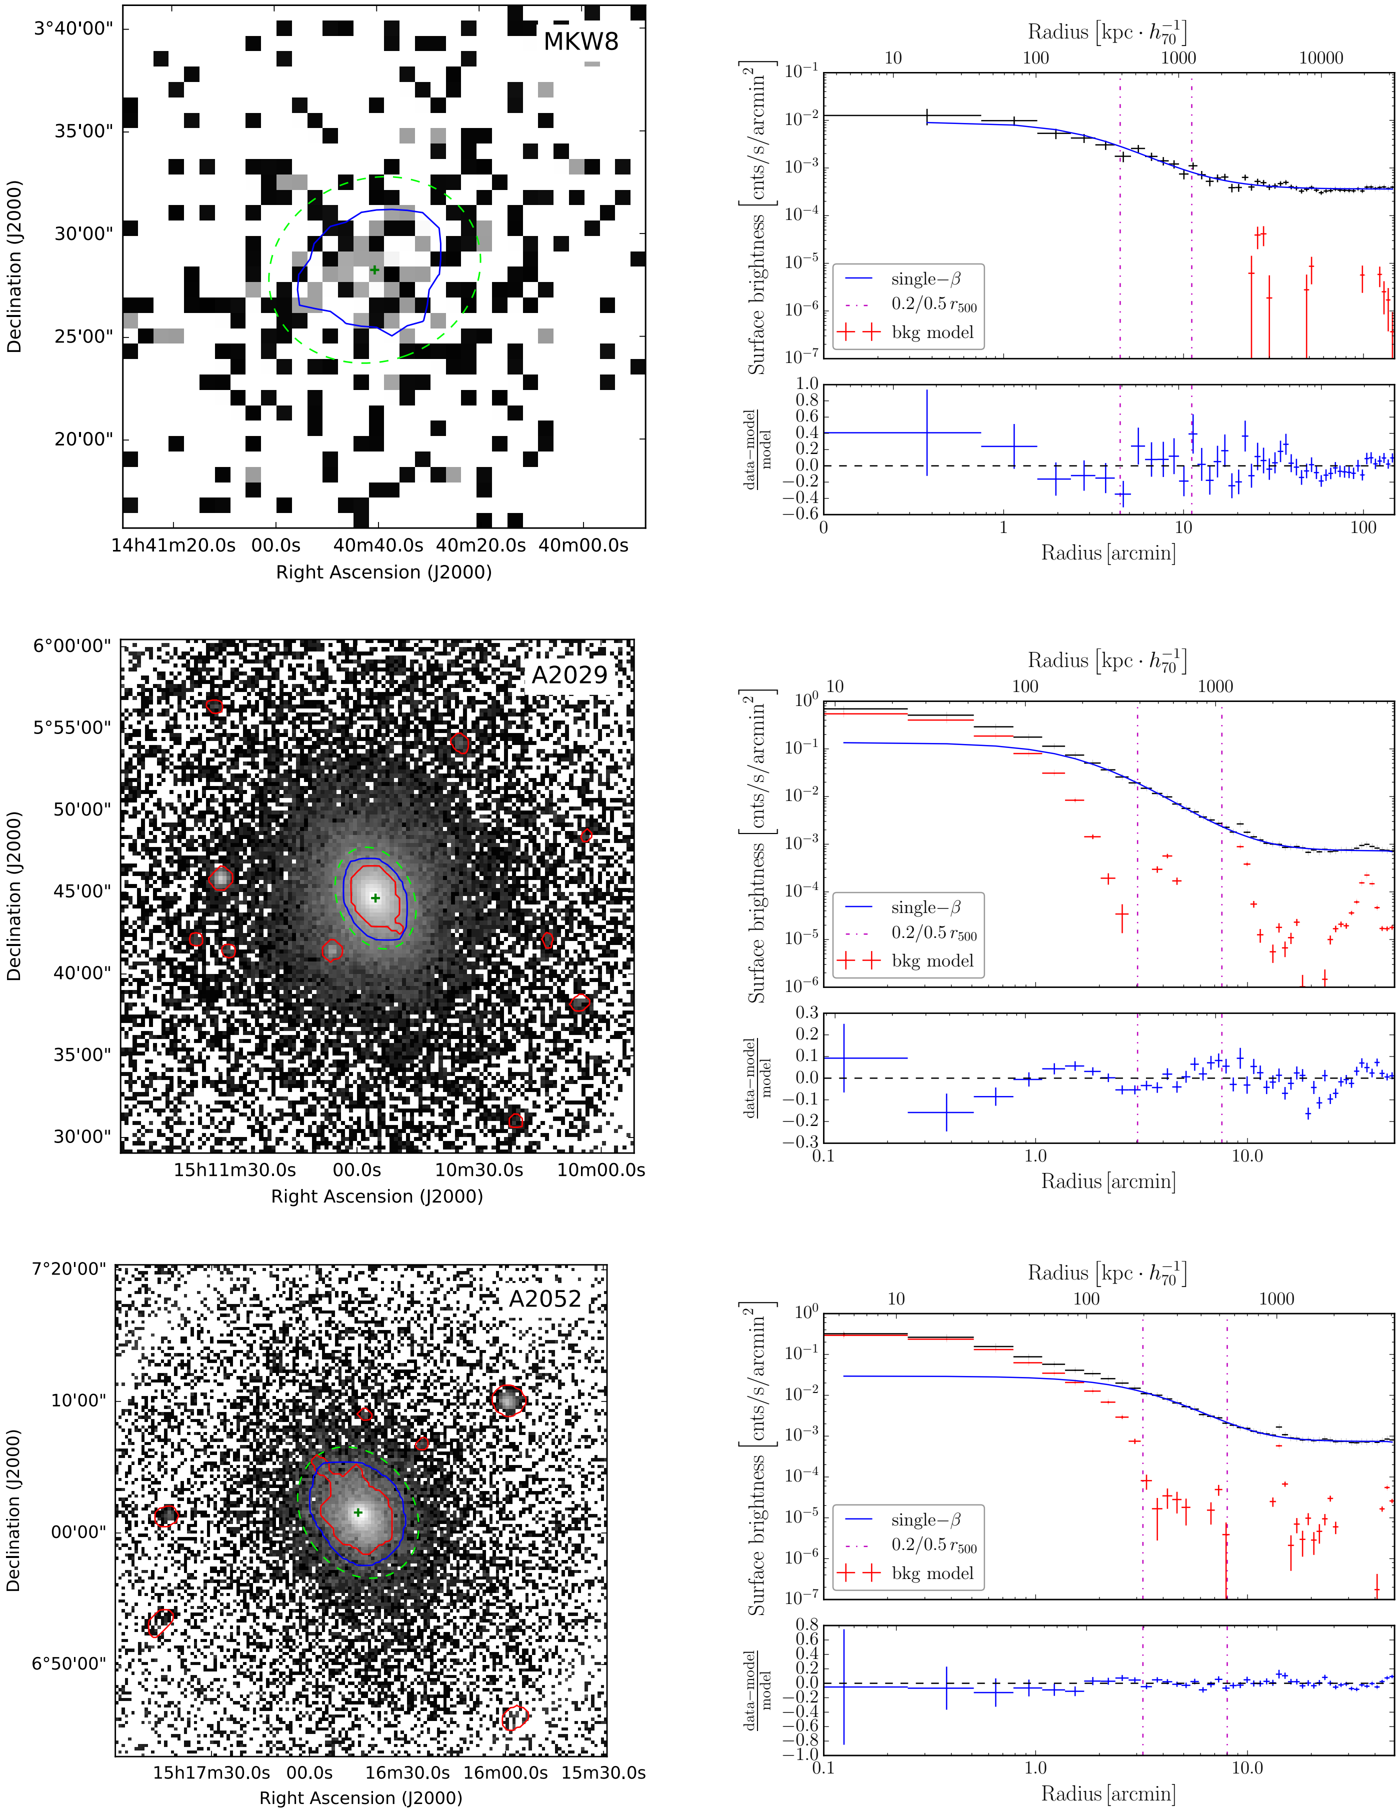


Fig. D.1: Continued.

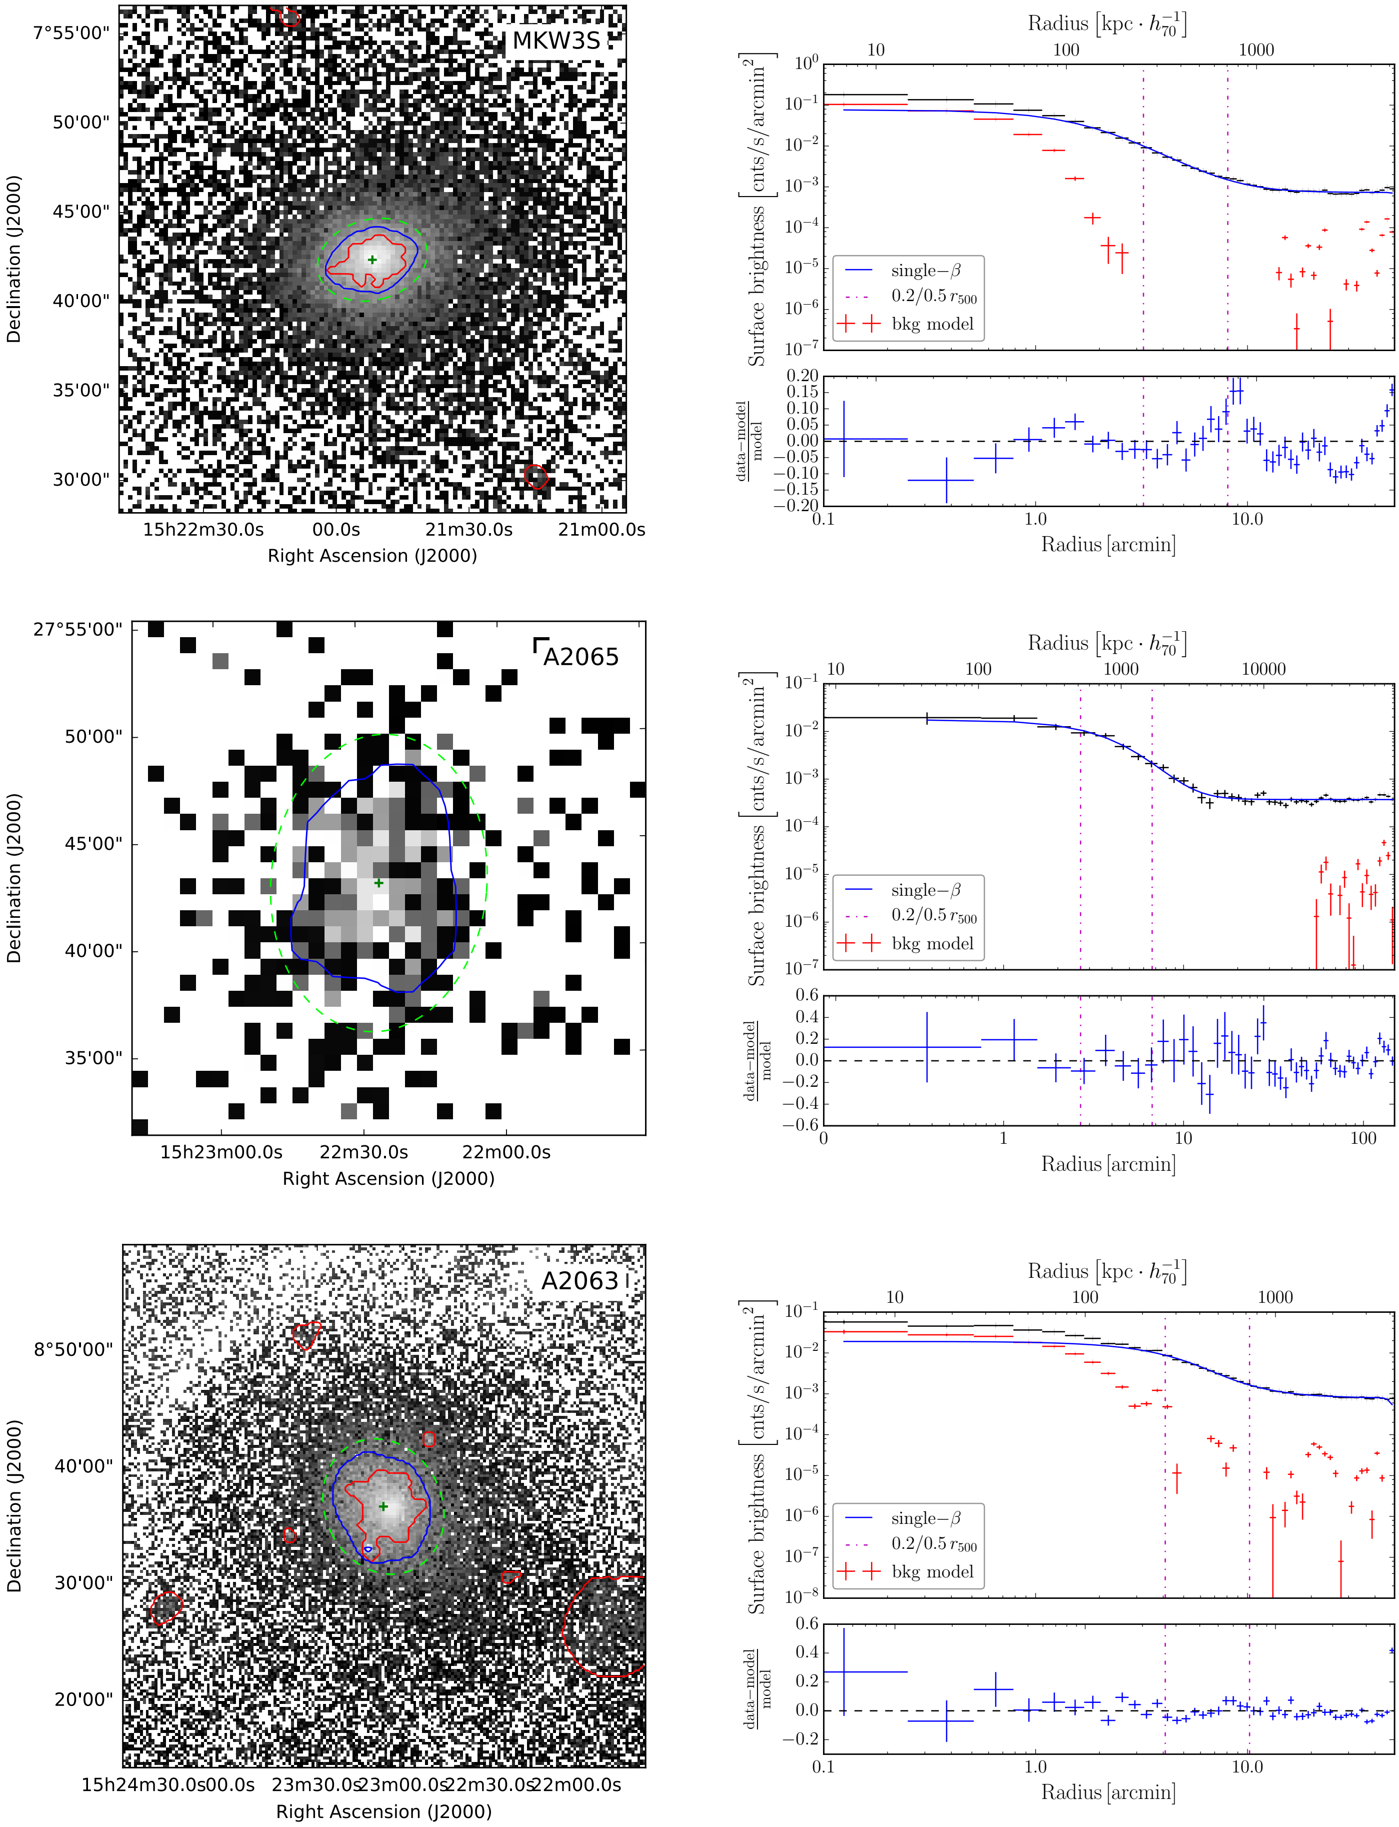


Fig. D.1: Continued.

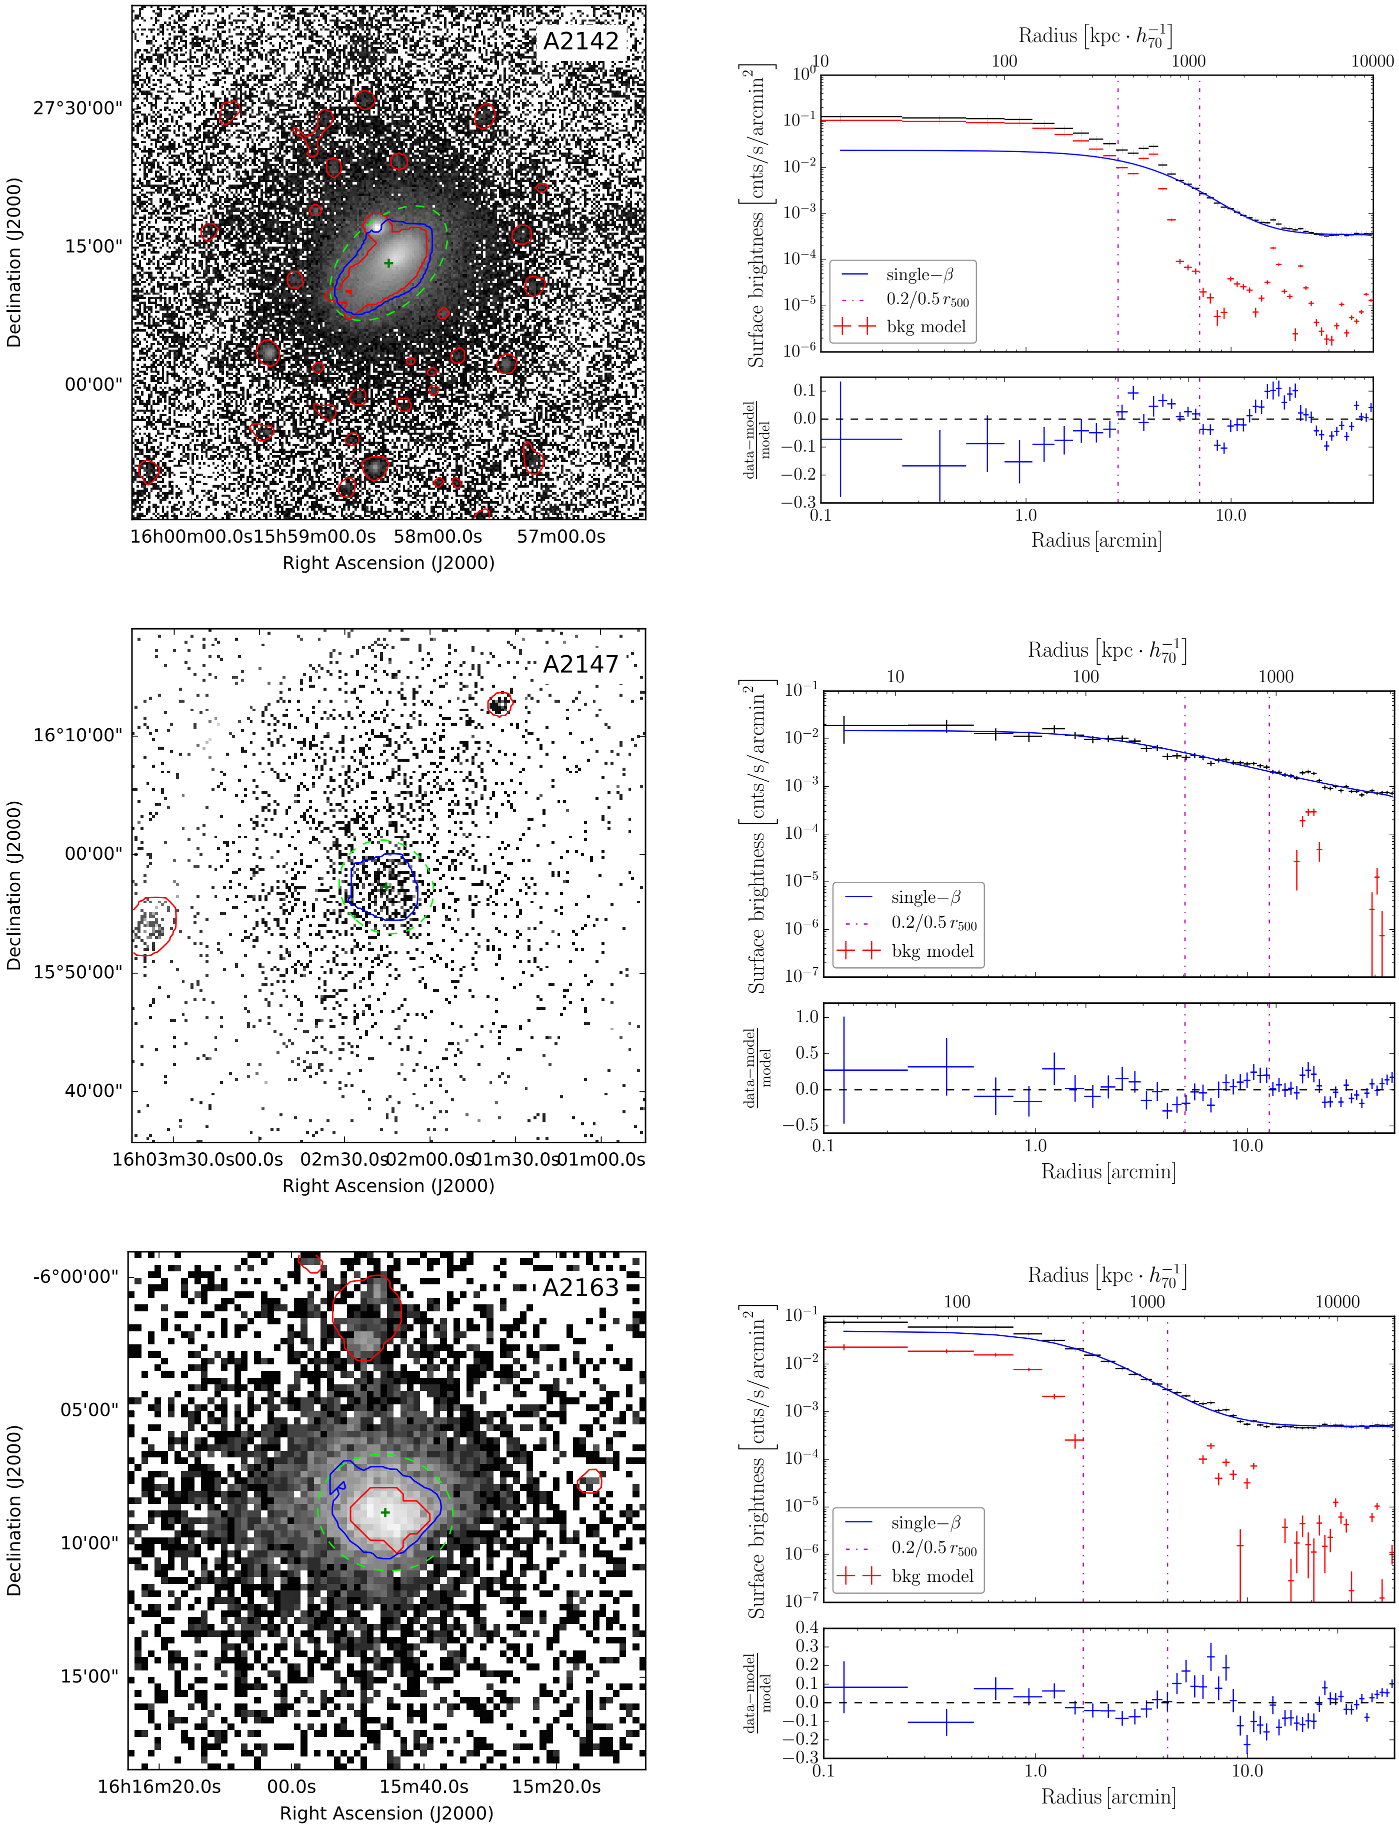


Fig. D.1: Continued.

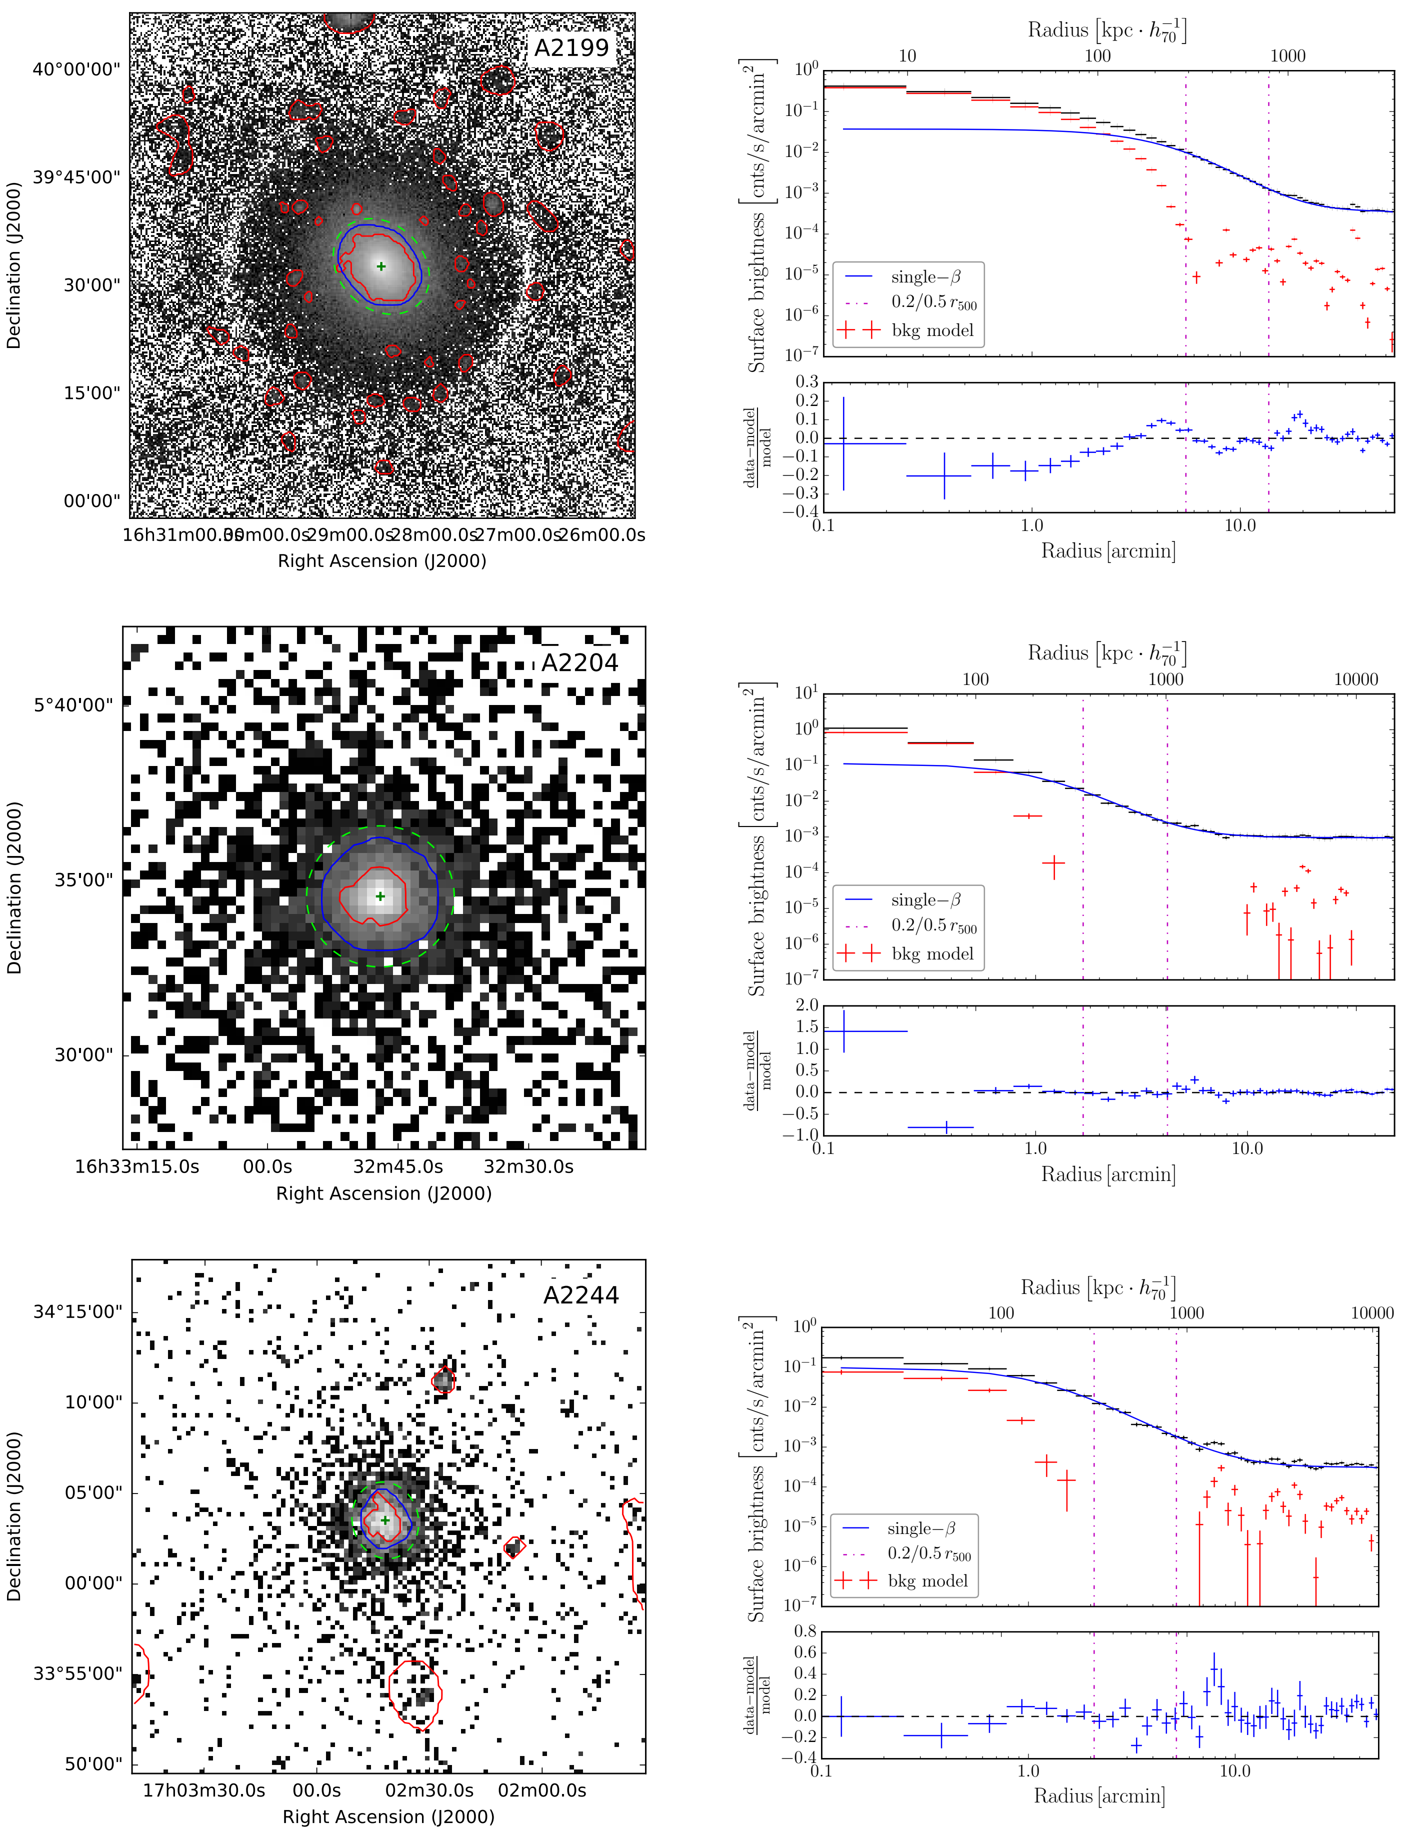


Fig. D.1: Continued.

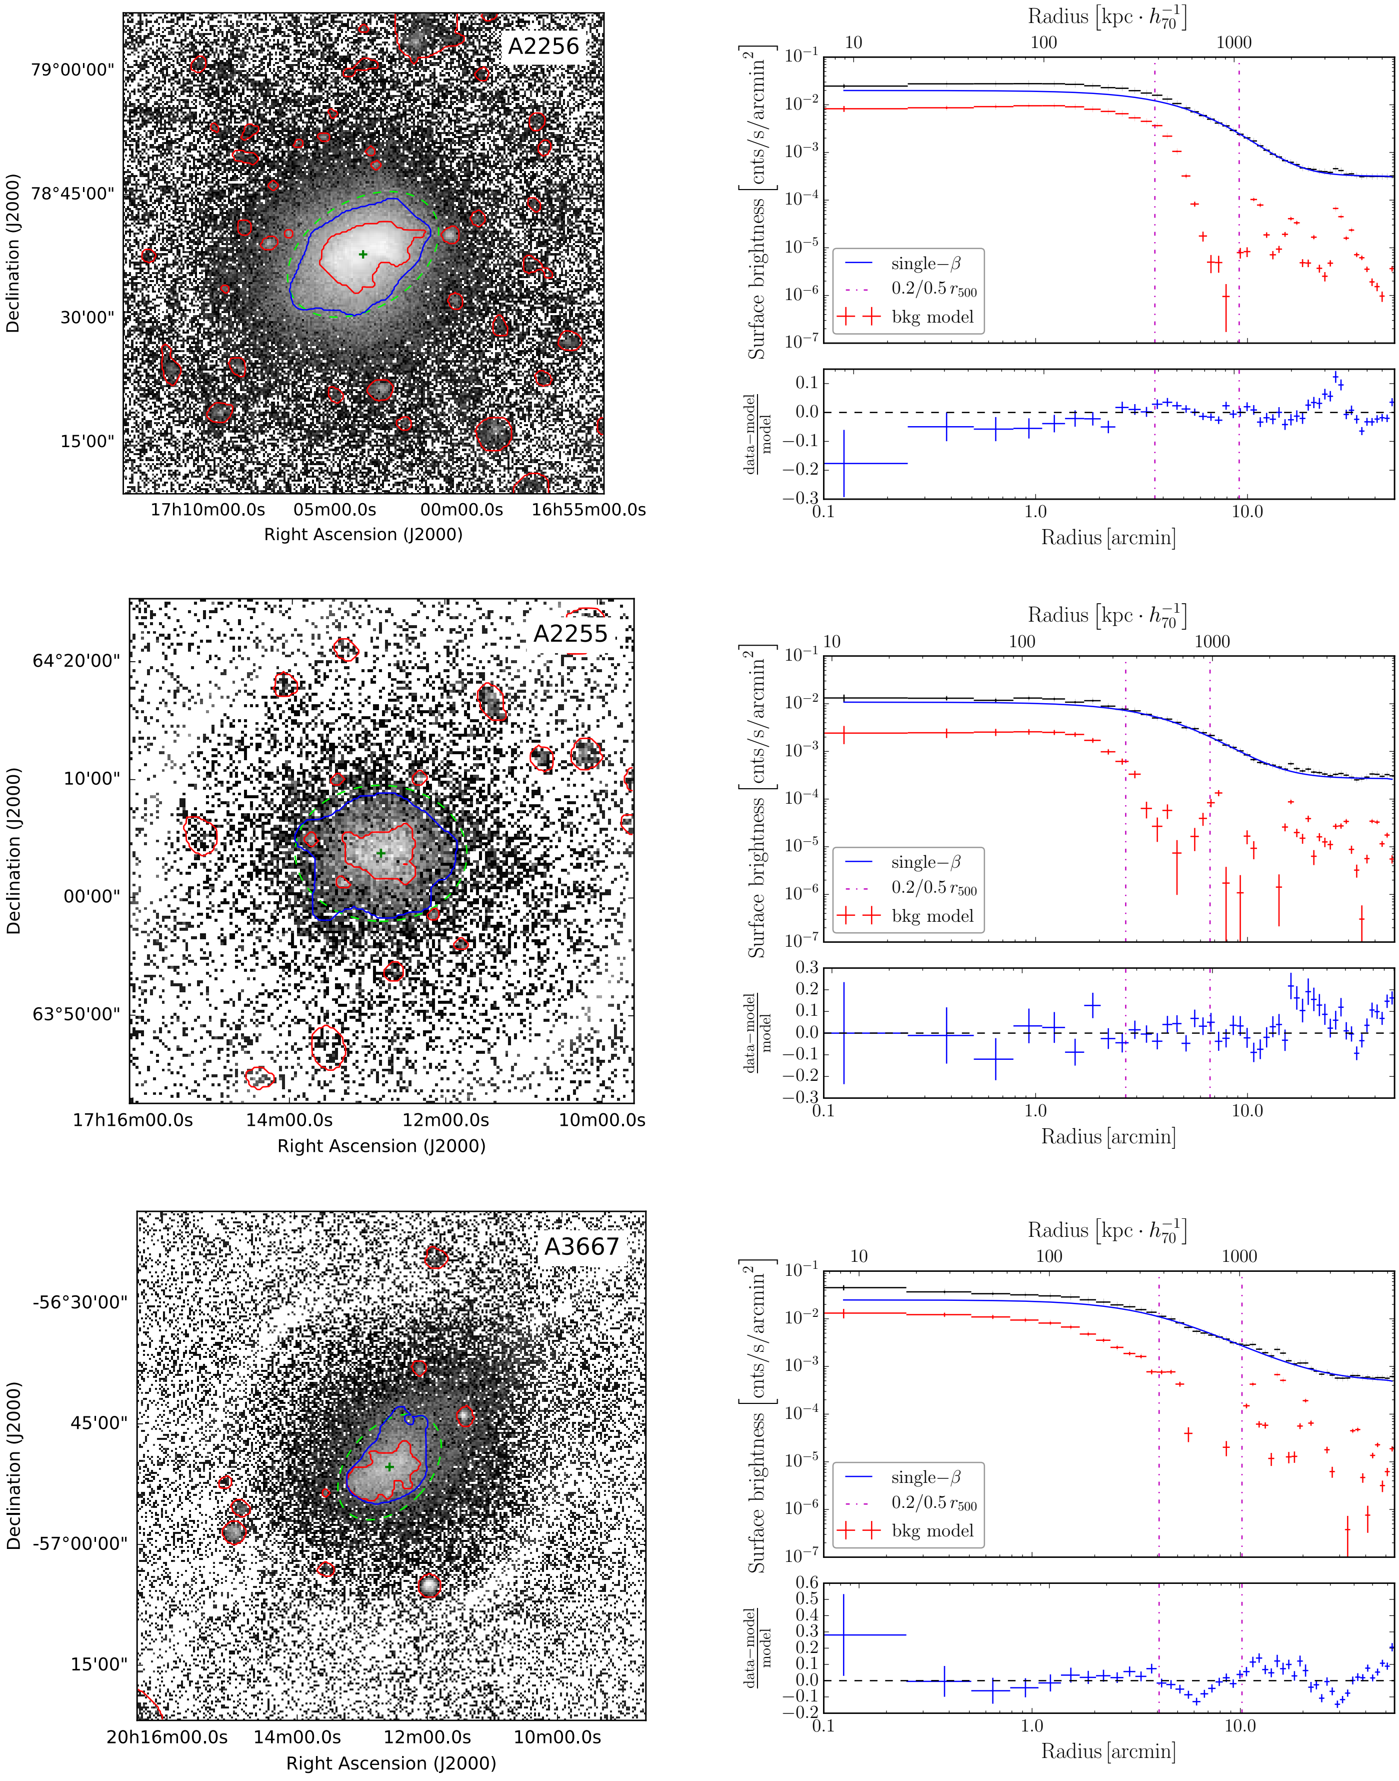


Fig. D.1: Continued.

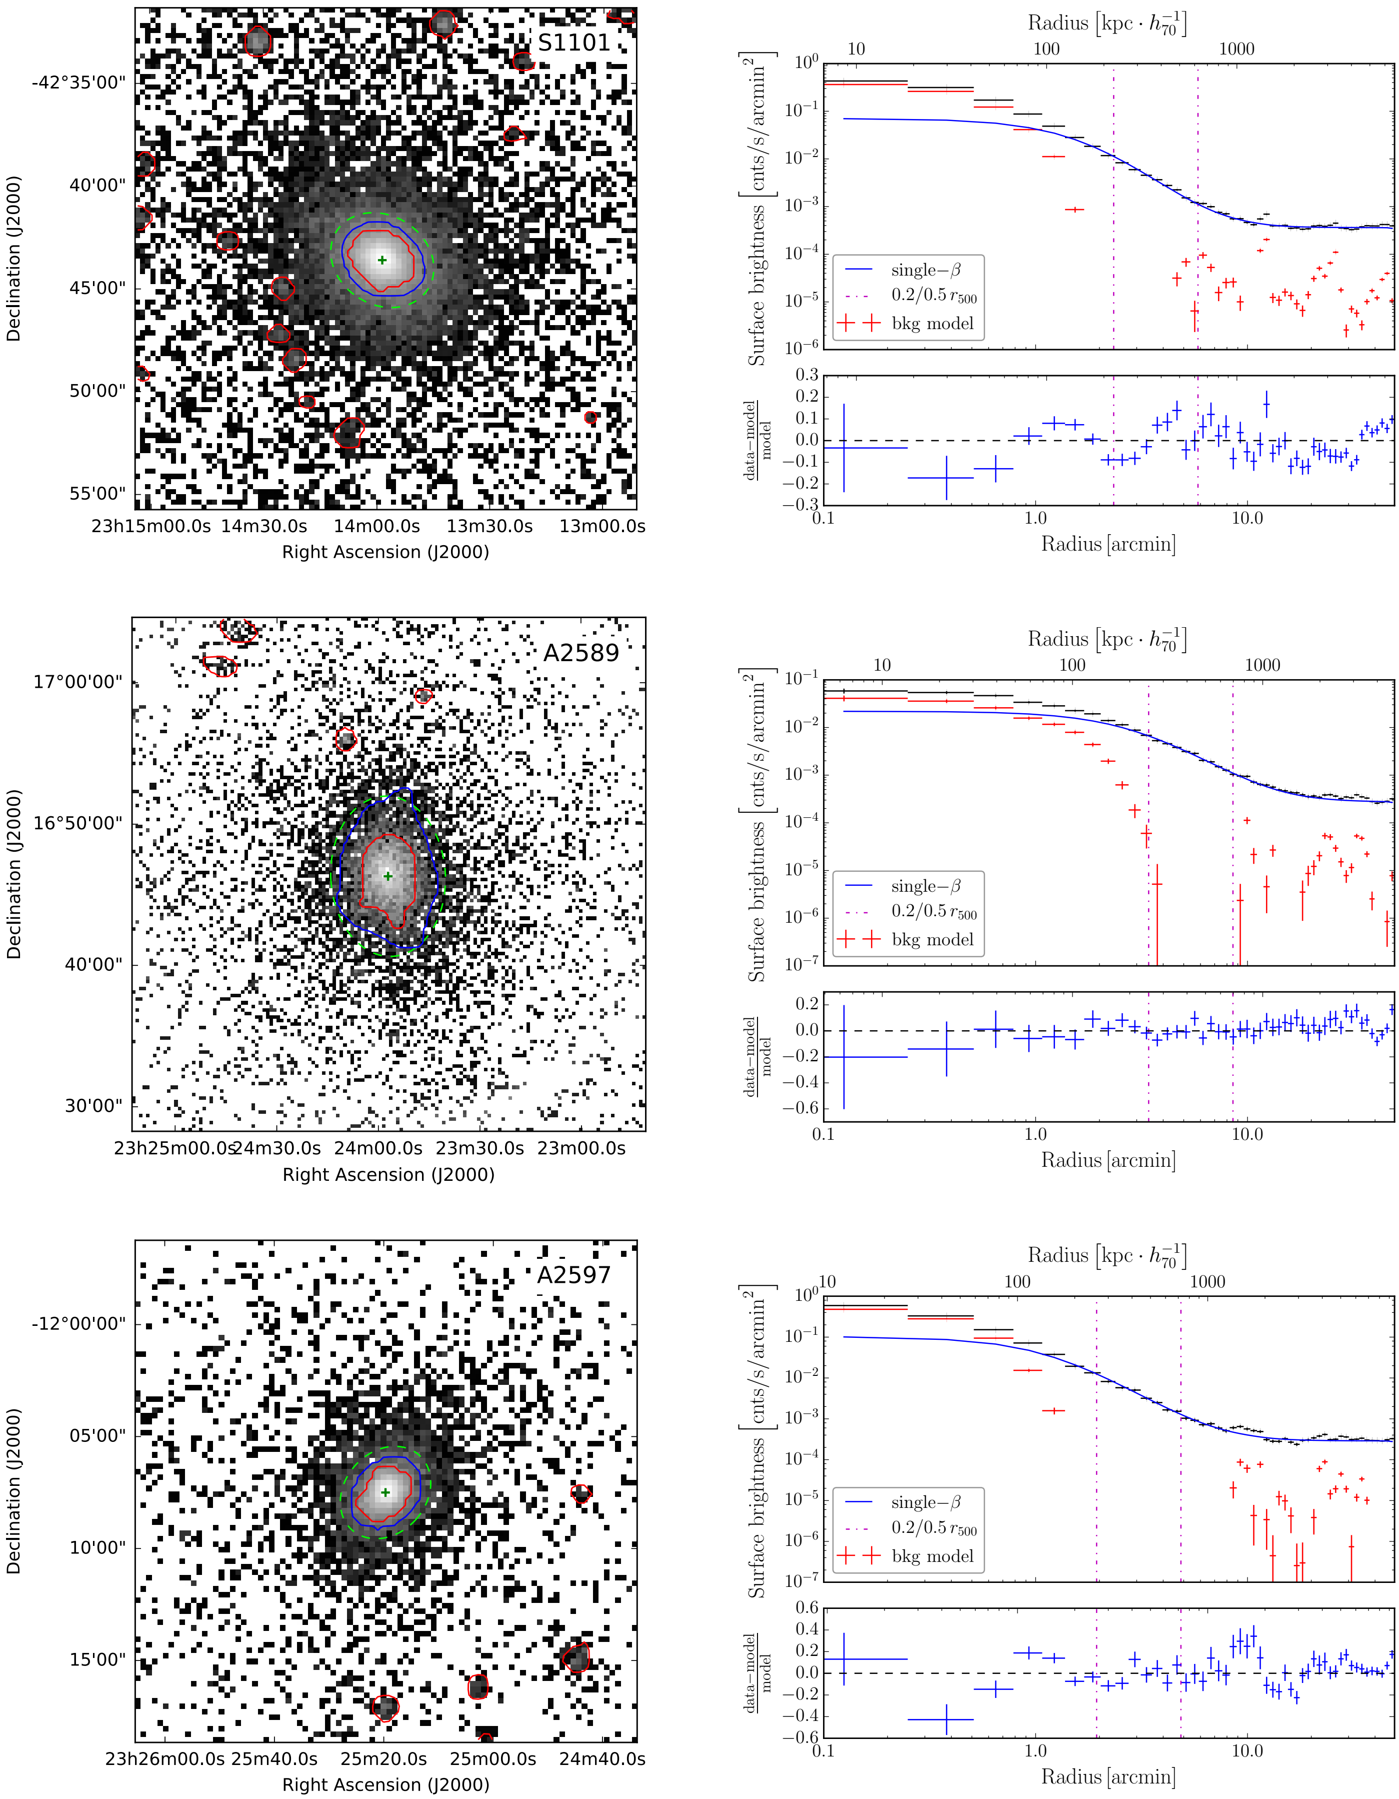


Fig. D.1: Continued.

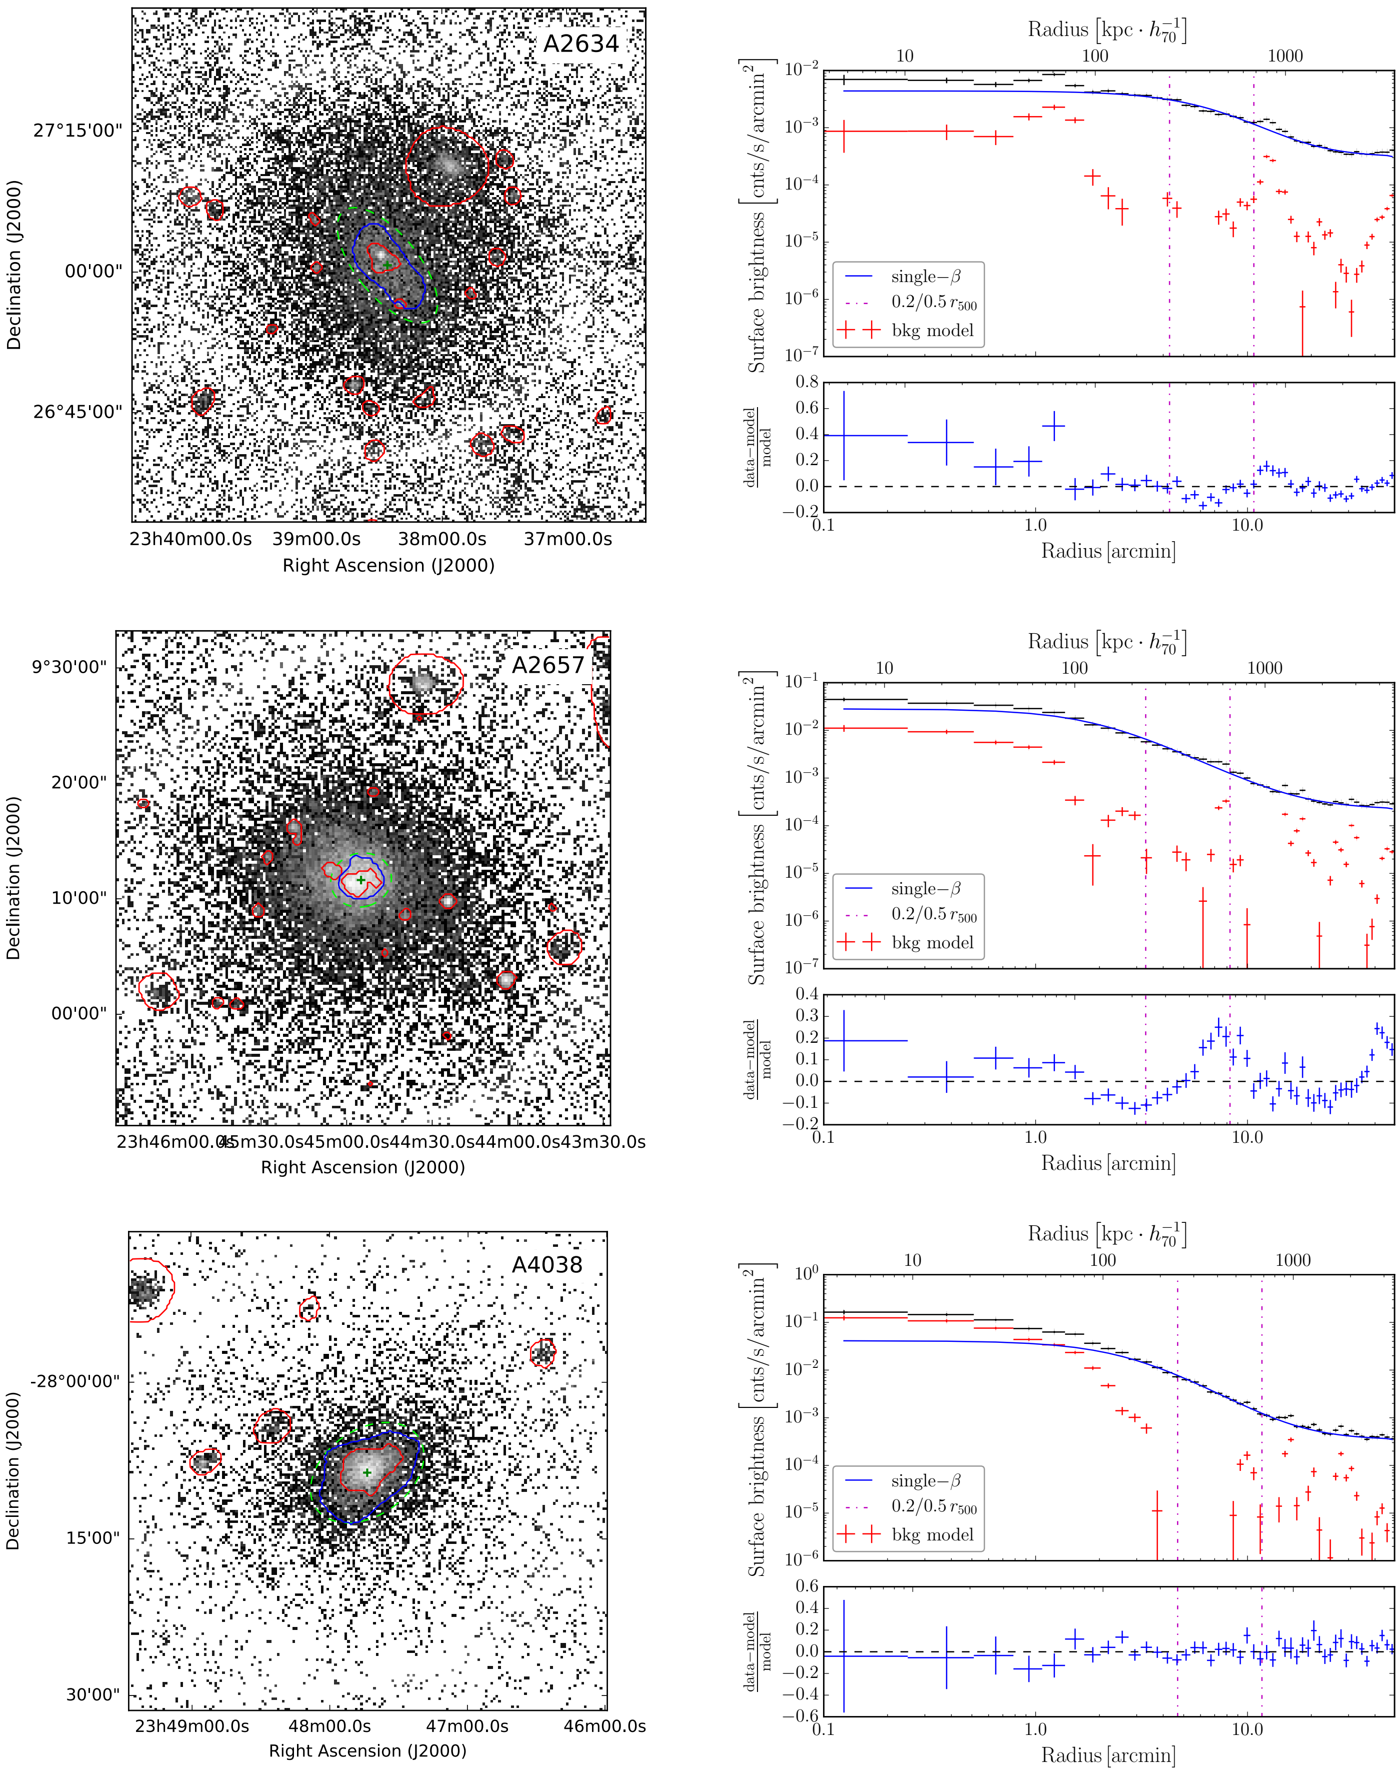


Fig. D.1: Continued.

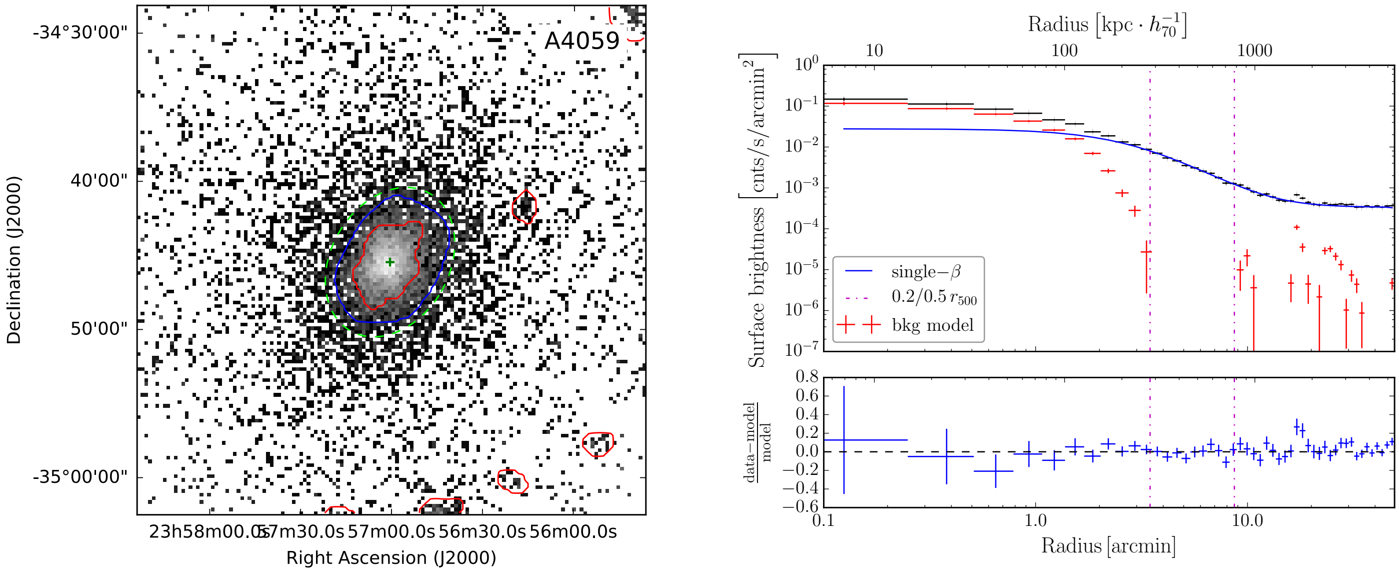


Fig. D.1: Continued.
